# Supplementary material for: Language-integrated provenance by trace analysis
Source: arXiv:1905.02051 source file (2019-05-06)
Supplement: Supplementary file 1 [file appendix.tex]

\section{Overview}\label{sec:tlinks-overview}
The implementations of \WLinks and \LLinks are separate extensions of \Links.
This does not have a deep technical reason; they could coexist in a single language.
Indeed, \citet{Programming2018StolarekC} have shown how to implement both where-provenance and lineage in \Haskell using similar query transformations. %  , using the \DSH library \citep{IFL2010GiorgidzeGSW}.
It is even conceivable to apply both transformations to the same query.\footnote{where-provenance first, then lineage, otherwise the former would try to annotate annotations from the latter. The latter applies only to list constructors, which the former ignores.}
We thus claim that language-integrated provenance satisfies Requirement 1: ``support for different types of provenance'' \citep{Festschrift2013GlavicMG}.
However, the situation is not ideal.
Extending \Links in the manner of \WLinks and \LLinks requires changes to the parser, typechecker, and interpreter.
This is not something regular programmers should be expected to do.
The situation in \Haskell is not much better.
While \citet{Programming2018StolarekC} did not need to change the implementation of \Haskell, they did have to change the implementation of \DSH to, among other things, ``implement our own type checking for some fragments of the lineage transformation''.
% \DSH being an embedded domain-specific language, we consider \Haskell to be its meta-language, almost the same as \OCaml being the meta-language of \Links.
We would much prefer programmers be able to define their own forms of provenance without changing the implementation of their query language (embedded or not).

\TLinks takes inspiration from work on \emph{slicing} database queries \citep{cheney14ppdp} and (imperative) functional programs \citep{ICFP2012PereraACL,Ricciotti:2017:IFP:3136534.3110258}.
The common theme in this line of work is tracing execution to have enough information to answer questions about which parts of the program are responsible for which parts of the output.
They define augmented evaluation procedures that not only produce a value, but also a trace of the execution.
They also define forward and backward slicing, which are two ways to analyze the traces to see which part of the program is responsible for which part of the output and the other way round.

Recent work by \citet{misinterpretingsql} is closely related to \TLinks and in some ways more advanced.
The standard semantics of \SQL queries is to produce a value when run on a database.
\citet{misinterpretingsql} show different interpretations of \SQL queries that produce where-provenance and lineage of a query.
Unlike in \TLinks and in the slicing work, there is no single tree structured trace.
They essentially decompose the single trace into two parts: a dynamic part which records control flow decisions the database system needs to make depending on the data; and a static part that is just the structure of the query.
Their work also extends to \SQL features like grouping and aggregation that are not implemented in \Links, let alone traced in \TLinks.

In both of these lines of work, queries do not have access to the trace and it is not the query language that is used to interpret the traces.
Instead, both the trace and its analysis live outside of the program.
In contrast, \TLinks traces are a recursive datatype in the language itself.
We can wrap a piece of code in a \lstinline|trace| block and get back a value --- the trace that represents the code's execution.
We can write (recursive) functions that analyze traces and extract information, like from any other datatype.
We can even combine multiple different trace analyses.

The key constraint is designing the traces and trace analysis functions such that when we compose analysis and tracing of some code and the result has a query type, we can compile the code to a bounded number of \SQL queries.
That is, assuming normalization terminates, which we do not prove.
Queries can be constructed at runtime to be arbitrarily large.
To deal with arbitrarily large traces, we need to write recursive trace analysis functions.
Recursive functions do not in general normalize --- they may loop.
We currently do not enforce termination through means like checking syntactically for structural recursion.

The rest of this section gives a high-level overview of \TLinks's features.
We describe type-level computation, how to make term-level decisions based on types, generic operations on records, and what traces look like by example.

\subsection{Type functions and Typerec}\label{sec:overview-typerec}
Sometimes, it is useful to make decisions based on types.
\TLinks has two language features to support this: \lstinline{Typerec} on the type-level and \lstinline{typecase} on the term-level.
Recall the lineage translation on types $\mathfrak{L}\llbracket \cdot \rrbracket$ (Figure \ref{fig:llinks-type-translation}) that we used to define what lineage-annotated types look like:
base types are translated to themselves, for list types we recursively translate the type argument and add the actual lineage annotations, and records are just recursively translated.
For \LLinks this was implemented on the meta-level in \OCaml.
In \TLinks we can use \lstinline{Typerec} to define such a traversal:
\begin{lstlisting}
Typerec a (Bool, Int, String,
           $\lambda$b b'. [$\langle$data:b', lineage:[$\langle$%table%:String, row:Int$\rangle$]$\rangle$],
           $\lambda$r r'. $\langle$r'$\rangle$)
\end{lstlisting}
You can read the snippet above as a fold over the type \lstinline|a|.
If \lstinline|a| is one of \lstinline{Bool}, \lstinline{Int}, or \lstinline{String} we return the same.
On the second line we have a type function of two arguments that defines what to do if \lstinline|a| is a list type.
It is called with the first argument \lstinline|b| bound to the element type of \lstinline|a| and the second argument \lstinline|b'| bound to the result of applying the \lstinline{Typerec} expression recursively to the element type of \lstinline|a|.
The result in our case is a list type where the elements are records containing recursively traversed lineage-annotated types and a list of lineage annotations.
The third line defines another type-level function.
It gets called when \lstinline|a| is a record type and gets passed the original row, as well as the row obtained by recursively evaluating the \lstinline{Typerec} expression on all field types.
In our case we want to recursively go through records, so we return a record with row \lstinline|r'|.

\subsection{Type-directed programming with typecase}\label{sec:overview-typecase}
On the term-level we have \lstinline{typecase} to make decisions based on types.
A typical application is overloading functions, for example for pretty printing.
Perhaps the simplest use case is to define a default value at any type, as below.
\begin{lstlisting}
default : $\forall$a:Type.a
default = $\Lambda$a:Type.typecase a of
  Bool   => false
  Int    => 0
  String => ""
  List b => []
\end{lstlisting}
This snippet defines \lstinline|default|, a polymorphic value that has any type in a universe of base types and list types.
It is defined as a type abstraction $\Lambda$ that binds type \lstinline|a| and then pattern matches on the shape of \lstinline|a| using \lstinline|typecase|.
The base type branches return some typical default value.
The list branch binds element type \lstinline|b| and returns the empty list of type \lstinline|List b|.
Using this definition we have \lstinline|default Int == 0| and \lstinline|default (List (List Bool)) == []|.

In \TLinks the universe of types that can be inspected by \lstinline|typecase| additionally includes record types and trace types.
Ad-hoc polymorphism is generally useful, but for us it is crucial for writing generic functions that can later be applied to analyze traces of queries of any type.
This and the next feature are what allows us to write a trace analysis function once and then use the same function to compute provenance of queries with any type.

\subsection{Generic record programming}
Since we want to be able to write a single trace analysis function and apply it to a variety of queries, we need to be able to work generically with records.
\TLinks supports two generic operations on records: mapping and folding.

For example, we can convert a record to a record of strings, by mapping a polymorphic \lstinline|show| function over it like so:
\begin{lstlisting}
rmap show $\langle$a=true, b=[false]$\rangle$
\end{lstlisting}
with the following result: \lstinline|$\langle$a="true", b="[false]"$\rangle$|.

The expression in function position, \lstinline|show| in this case, must have the following polymorphic function type: $\forall \alpha. \alpha \rightarrow F \alpha$, where $F$ is a type-level function.
In our example, $F$ is the constant type-level function $\lambda \alpha: \mathit{Type}. \mathtt{String}$.
For closed records, the result type of a record map expression is another record type with the type-level function $F$ applied to the labels' types.
For open records, that is records whose row contains a row variable $\rho$, we keep track of the fact that we apply a type-level function to the labels' types using the type-level row map operation \lstinline|Rmap|.
Given a type-level function $F$ and a row type $R$, \lstinline|Rmap $F$ $R$| represents the row type that applies $F$ to all of $R$'s labels' types.
For example, the following types are all equivalent:
\begin{lstlisting}
  {a: String, b: String}
= Record (a: String, b: String)
= Record (a: ($\lambda$a.String) Bool, b: ($\lambda$a.String) (List Bool))
= Record (Rmap ($\lambda$a.String) (a: Bool, b: List Bool))
= ($\lambda$r.Record (Rmap ($\lambda$a.String) r)) (a: Bool, b: List Bool)
\end{lstlisting}

The second generic record operation is folding.
We will need this to combine annotations from the fields of a record, for example in the lineage implementation in Section~\ref{sec:taf-lineage}.
For this introduction, let us assume we wanted to count the number of times \lstinline|true| appears in a record.
Given a polymorphic \lstinline|countTrue| function, we could map it over the record, and then use a record fold operation to further reduce the resulting homogeneous record into the final sum:
\begin{lstlisting}
rfold (+) 0 (rmap countTrue {a=true,b=[true,false],c=5})
\end{lstlisting}
The result of mapping is \lstinline|{a=1,b=1,c=0}| and folding with addition and initial accumulator 0 results in 2.
As the order of labels in records is undefined, the order of traversal by \lstinline|rmap| and \lstinline|rfold| is undefined too.
Since we only have pure functions in queries, the order of execution makes no difference to \lstinline|rmap|.
When using \lstinline|rfold| however, it is best to use a commutative combining function.

During \TLinks query compilation, \lstinline|rmap| and \lstinline|rfold| are unrolled based on types.
This works because queries do not contain free (row) variables and all record types that appear in a query directly are closed (they are either literal record constructions, or come from tables which have fixed columns).

% We only allow folding of homogenous records, or more precisely, records whose type is equivalent to a record type obtained by row map of a constant function over a row type.
% Here is how given a record of pairs we could sum up all of the second components:
% \begin{lstlisting}
% snd : $\forall$r.{snd: Int | r} -> Int
% snd r = r.snd

% sumSnds : $\forall$r.{ | Rmap ($\lambda$r'.{snd: Int | r'}) r} -> Int
% sumSnds r = rfold (+) 0 (rmap snd r)
% \end{lstlisting}

% \stefan{what was the example that Sam asked about regarding homogeneity? Was it mapping/folding with \lstinline|snd|? like \lstinline|\{a:(Bool, Int), b:(String, Int)\}|}
% \stefan{Ugh. Can we even do that? What would the type look like of a sumSnds function? It takes a record whose fields are constrained. I'm not sure we can express that.}

% \stefan{urweb (different primitives), purescript (rowtolist and fundeps), encoded records = encoded operations, probably, like in idris}

\subsection{Traces of queries}

What exactly do these traces look like?
We answer this in detail in Section~\ref{sec:self-tracing-queries}.
For now, let us look at a few examples.
The trace of the literal 42 is \lstinline{Lit 42}.
\lstinline{Lit} is a constructor of the built-in type \lstinline|Trace|.
Tracing a list of literals like \lstinline|[42, 43]| results in a list of traces like \lstinline|[Lit 42, Lit 43]|.
And tracing a record \lstinline|{a=true,b=42}| results in a record of traces \lstinline|{a=Lit true,b=Lit 42}|.
This is perhaps the most important aspect of traces in \TLinks: the trace of a list is a list of traces and, similarly, the trace of a record is a record of traces.
Projection is not recorded in traces: \lstinline|{a=true,b=42}.a| results in the trace \lstinline|Lit true|.
Tracing tables annotates all cells.
For example, the trace of \lstinline|presidents| from Figure~\ref{fig:inaugurations-db} would look something like this (modulo \lstinline|oid|s):
\begin{lstlisting}
[{nth=Cell {%table%="presidents", column="nth", row=432, data=1},
  name=Cell {%table%="presidents", column="name", row=432,
             data="George Washington"}},
 ...,
 {nth=Cell {%table%="presidents", column="nth", row=564, data=44},
  name=Cell {%table%="presidents", column="name", row=564,
             data="Barack Obama"}},
 {nth=Cell {%table%="presidents", column="nth", row=149, data=45},
  name=Cell {%table%="presidents", column="name", row=149,
             data="Donald Trump"}}]
\end{lstlisting}
That is, data from table cells is annotated with the \lstinline|Cell| constructor which carries table name, column name, and row identifier (we use \lstinline|oid|s again) alongside the actual data.
The other \lstinline{Trace} constructors are: \lstinline{Lit} for values from the query itself rather than the database; \lstinline{If} for the result of an \lstinline{if-then-else} annotated with subtraces of the conditional expression and the branch taken; \lstinline{For} for values that were produced by a comprehension, recording a trace of the input and the output; and traces of primitive operators like \lstinline{==} and \lstinline{+} that record subtraces for their arguments.

Polymorphic operations record at which type they were applied.
For example, the trace for \lstinline{5 == 7} is \lstinline!OpEq Int {left=Lit 5, right=Lit 7}!.
In addition to the left and right subtraces, we record that in this case equality was applied at type \lstinline!Int!.
Comprehensions are also polymorphic and record the type of the input collection's elements.

\begin{figure}
\begin{lstlisting}
[{name=
   For{in={name=Cell{%table%="agencies", column="name",
                     row=?, data="EdinTours"},
           phone=Cell{%table%="agencies", column="phone",
                     row=?, data="4121200"},
           based_in=Cell{%table%="agencies", column="based_in",
                     row=?, data="Edinburgh"}},
       out=
     For{in={type=Cell{%table%="externalTours", column="type",
                       row=?, data="boat"},
             name=...,
             price=...,
             destination=...},
         out=
       If{cond=OpAnd{left=
                 OpEq String {left=Cell{%table%="agencies",
                                        column="name",
                                        row=?,
                                        data="EdinTours"},
                              right=Cell{%table%="externalTours",
                                         column="name",
                                         row=?, data="EdinTours"}},
                     right=
                 OpEq String {left=Cell{%table%="externalTours",
                                        column="type",
                                        row=?, data="boat"},
                              right=Lit "boat"}},
          branch=Cell{%table%="agencies", column="name",
                      row=?, data="EdinTours"}}}}
  phone=...},
 {name=..., phone=...},
 ...]
\end{lstlisting}
  \caption{Partial trace of the boat tours query.}
  \label{fig:boattours-trace}
\end{figure}

Figure \ref{fig:boattours-trace} shows a partial trace of the larger (but really still quite small) boat tours query.
It has almost the full trace for the name field of the first result row.
We see how nested \lstinline|for| comprehensions lead to nested \lstinline|For| trace constructors, and nested comparisons in the conditional expression lead to nested \lstinline|OpAnd| and \lstinline|OpEq| traces.
Note that this is for illustration purposes only.
We do not intend to ever actually construct the whole trace.
We expect to compose the self-tracing query with a trace analysis function and evaluate away all trace constructors during query normalization.

We use \lstinline{tracecase} to pattern match, or rather case split, on trace constructors.
The branches for \lstinline|For| and \lstinline|OpEq| bind an additional type variable.
For example, the snippet below would evaluate to \lstinline|f Int (Lit 5)|:
\begin{lstlisting}
tracecase OpEq Int {left=Lit 5, right=Lit 6} of
  Lit x    => ...
  If x     => ...
  For a x  => ...
  Cell x   => ...
  OpEq a x => f a x.left
  OpPlus x => ...
\end{lstlisting}

This concludes the informal overview of \TLinks features.
The next sections describe the syntax and static semantics of \TLinks, including normalization to nested relational calculus, and the self-tracing transformation.
If you are inclined to skip the technical details for now, Section \ref{sec:trace-analyses} shows \TLinks in action.
There we define trace analysis functions to extract provenance from traces.

\section{Syntax \& semantics}
\label{sec:trace-syntax-semantics}

\TLinks is meant to eventually be implemented as an extension to \Links.
However, the language design described here is more closely based on \lamiml, a core calculus devised by \citet{Harper:1995:CPU:199448.199475}.
% based on earlier work by \citet{constable82}.
% \stefan{(I can't actually find this tech report anywhere.)}
This presentation of the typing rules in particular is based on a later presentation of \lamiml by \citet{crary_weirich_morrisett_2002}.
We modify the core of \lamiml to accommodate \Links features like row types, records, and lists.
To simplify the presentation, \TLinks is entirely pure but we imagine that an eventual implementation would use effect types much as \Links does \citep{TLDI2012LindleyC} to distinguish database-executable query expressions from other programs.

\begin{figure}[t]
  \footnotesize
  \[
    \begin{array}{lrcl}
      \text{Contexts} & \Gamma & \Coloneqq & \cdot \mid \Gamma, \alpha: K \mid \Gamma, x: A \\
      \\
      \text{Kinds} & K & \Coloneqq & \mathit{Type} \mid \mathit{BaseType} \mid \mathit{Row} \mid \mathit{BaseRow} \mid K_1 \rightarrow K_2 \\
      \\
      \text{Constr.} & C, D & \Coloneqq & \texttt{Bool}^* \mid \inttyc \mid \texttt{String}^* \mid \alpha \mid \lambda \alpha: K.C \mid C\ D \\
                   & & \mid & \texttt{List}^*\ C \mid \texttt{Record}^*\ S \mid \texttt{Trace}^*\ C \\
                   & & \mid & \kw{Typerec}~ C~ (C_B, C_I, C_S, C_L, C_R, C_T) \\
      \text{Row constr.}  & S   & \Coloneqq & \cdot \mid l : C; S \mid \rho \mid \kw{Rmap}\ C\ S \\
      \\
      \text{Types} & A, B & \Coloneqq & \texttt{T}(C) \mid \texttt{Bool} \mid \intty \mid \texttt{String} \mid A \rightarrow B \\
                   & & \mid & \texttt{List}\ A \mid \texttt{Record}\ R \mid \texttt{Trace}\ A \mid \forall \alpha:K.A \\
      \text{Row types}  & R   & \Coloneqq & \cdot \mid l : A; R \\
      \\
      \text{Terms} & L, M, N & \Coloneqq & c \mid x \mid \lambda x:A.M \mid M\ N \mid \Lambda \alpha:K.M \mid M\ C \\
                   & & \mid & \kw{fix}~f:A.M \mid \kw{if}~L~\kw{then}~M~\kw{else}~N \mid M + N \mid M == N \\
                   & & \mid & \langle \rangle \mid \langle l = M; N \rangle \mid M.l \mid \kw{rmap}^S~L~M \mid \kw{rfold}^S~L~M~N \\
                   & & \mid & [] \mid [M] \mid M \concat N \mid \kw{for}~(x \leftarrow M)~N \mid \kw{table}~n~\langle R \rangle \\
                   & & \mid & \texttt{Lit}\ M \mid \texttt{If}\ M \mid \texttt{For}\ C\ M \mid \texttt{Cell}\ M \mid \texttt{OpEq}\ C\ M \mid \texttt{OpPlus}\ M \\
                   & & \mid & \kw{tracecase}~M~\kw{of}~(x.M_L, x.M_I, \alpha.x.M_F, x.M_C, \alpha.x.M_E, x.M_P) \\
                   & & \mid & \kw{typecase}~C~\kw{of}\ (M_B, M_I, M_S, \beta.M_L, \rho.M_R, \beta.M_T) \\
    \end{array}
  \]
  \caption{The syntax of \TLinks.}
  \label{fig:tlinks-syntax}
\end{figure}

The syntax of \TLinks is shown in Figure \ref{fig:tlinks-syntax}.
We use a unified context $\Gamma$, mapping type variables $x$ to types $A$ and type variables $\alpha$ to kinds $K$.
Kinds include \textit{Type} and \textit{BaseType}, as well as \textit{Row} and \textit{BaseRow}, a row of base types.
Row constructors $S$ include row variables $\rho$.
We follow convention in using $\rho$ for row variables, but they really are just type variables with kind \textit{Row}.

\TLinks, like \lamiml, has two syntactic categories for type-like things: types~$A$ and constructors~$C$.
Types are what we usually understand as types, they categorize values.
Constructors are where type-level computation happens and they can be inspected by terms like \lstinline{typecase}, whereas types cannot be inspected.
% Constructors are basically an explicit sub-universe of analyzable types.

Types, unsurprisingly, contain base types, function types, list and record types.
For the sake of brevity, we will often write \lstinline{[$A$]} for \lstinline{List $A$} and $\langle R \rangle$ for \lstinline{Record $R$}.
In rules, we will also use the shorthand syntax $\kw{typecase}~C~\kw{of}$ $(M_B,$ $M_I, M_S, \beta.M_L, \rho.M_R, \beta.M_T)$ for
\begin{lstlisting}
typecase $C$ of
  Bool     => $M_B$
  Int      => $M_I$
  String   => $M_S$
  List $\beta$   => $M_L$
  Record $\rho$ => $M_R$
  Trace $\beta$  => $M_T$
\end{lstlisting} and similarly $\kw{tracecase}~M~\kw{of}~(x.M_L, x.M_I, \alpha.x.M_F, x.M_C, \alpha.x.M_E, x.M_P)$ for
\begin{lstlisting}
tracecase $M$ of
  Lit $x$    => $M_L$
  If $x$     => $M_I$
  For $\alpha$ $x$  => $M_F$
  Cell $x$   => $M_C$
  OpEq $\alpha$ $x$ => $M_E$
  OpPlus $x$ => $M_P$
\end{lstlisting}
Note that \lstinline|typecase| takes extra arguments to deal with records and traces compared to the feature preview in Section~\ref{sec:overview-typecase}.

The type \lstinline{T($C$)} in essence allows us to go from constructors to types.
Constructors duplicate some types, but not all, and add some type-level computation constructs.
We have base constructors, lists and records, which are all marked by a star that we will frequently omit if it does not matter whether we use a type or constructor or it is clear from the context.
\TLinks, unlike \lamiml, does not have a constructor for function types because we do not need it in queries---our main focus.
A type variable is a constructor, introduced either by a polymorphic type, see above, or by a type-level function.
Constructors also contain type-level function application and \lstinline{Typerec}.
Compared to the feature preview in Section~\ref{sec:overview-typerec}, \lstinline|Typerec| takes extra arguments for record and trace types.

Terms are mostly standard.
Constants $c$ are Boolean, number, and string literals.
Functions and term-level type abstraction are unary.
We only list the operators \lstinline|+| and \lstinline|==|, other standard operators work similarly.
Records are written in angle brackets, as are record types.
Record map and record fold take a row constructor $S$ as an argument.
We write this in superscript to indicate that the generic record operations are specialized by that row, see Section~\ref{sec:tlinks-normalization} for details.
The first term argument to \lstinline|rmap| and \lstinline|rfold| is a function.
The last term argument is a record whose row matches the superscript.
The middle argument to \lstinline|rfold| is the initial accumulator.
The constructors \lstinline|Lit|, \lstinline|If|, \lstinline|For|, etc.\ belong to the \lstinline|Trace| type.
The trace constructors \lstinline|For| and \lstinline|OpEq| carry not only a subtrace, but also a type constructor.
The \TLinks core language does not have variants, at this time.

\begin{figure}
  \footnotesize
  \begin{mathpar}
    \infer
    { }
    { \cdot \text{ is well-formed} }

    \infer
    {Γ ⊢ A : \textit{Type} \and x \notin \textit{Dom}(Γ)}
    {Γ, x : A \text{ is well-formed}}

    \infer
    {Γ \text{ is well-formed} \and \alpha \notin \textit{Dom}(\Gamma) }
    {Γ, \alpha : K \text{ is well-formed}}
  \end{mathpar}
  \caption{Well-formed contexts $\Gamma$.}
  \label{fig:well-formed-contexts}
\end{figure}

\begin{figure}
  \footnotesize
  \begin{mathpar}
    \infer
    { Γ \text{ well-formed} }
    { Γ ⊢ \texttt{Bool}^* : \textit{BaseType} }

    \infer
    { Γ \text{ well-formed} }
    { Γ ⊢ \inttyc : \textit{BaseType} }

    \infer
    { Γ \text{ well-formed} }
    { Γ ⊢ \texttt{String}^* : \textit{BaseType} }

    \infer
    { Γ(\alpha) = K }
    { Γ ⊢ \alpha: K }

    \infer
    { Γ, \alpha: K_1 ⊢ C: K_2 }
    { Γ ⊢ \lambda \alpha:K_1.C : K_1 \rightarrow K_2 }

    \infer
    { Γ ⊢ C : K_1 \rightarrow K_2 \\ Γ ⊢ D : K_1 }
    { Γ ⊢ C\ D: K_2 }

    \infer
    { Γ ⊢ C : \textit{Type} }
    { Γ ⊢ \texttt{List}^*\ C : \textit{Type} }

    \infer
    { Γ ⊢ S : \textit{Row} }
    { Γ ⊢ \texttt{Record}^*\ S: \textit{Type} }

    \infer
    { Γ ⊢ C : \textit{BaseType} }
    { Γ ⊢ \texttt{Trace}^*\ C : \textit{Type} }

    \infer
    { Γ ⊢ C : \textit{Type} \\
      Γ ⊢ C_B : K \\
      Γ ⊢ C_I : K \\
      Γ ⊢ C_S : K \\
      Γ ⊢ C_L : \textit{Type} \rightarrow K \rightarrow K \\
      Γ ⊢ C_R : \textit{Row} \rightarrow \textit{Row} \rightarrow K \\
      Γ ⊢ C_T : \textit{BaseType} \rightarrow K \rightarrow K }
    { Γ ⊢ \kw{Typerec}~C~(C_B, C_I, C_S, C_L, C_R, C_T) : K }

    \infer
    { Γ \text{ well-formed} }
    { Γ ⊢ \cdot : \textit{Row} }

    \infer
    { Γ ⊢ C:\textit{Type} \\ Γ ⊢ S : \textit{Row} }
    { Γ ⊢ l:C;S : \textit{Row} }

    \infer
    { Γ ⊢ C : \textit{Type} \rightarrow \textit{Type} \\ Γ ⊢ S : \textit{Row} }
    { Γ ⊢ \kw{Rmap}\ C\ S : \textit{Row} }
  \end{mathpar}

  \caption{Constructor and row constructor kinding.}% formation $Γ ⊢ C : K$.}
  \label{fig:constructor-formation}
\end{figure}

\begin{figure}
  \footnotesize
  \begin{mathpar}
    \infer
    { Γ ⊢ C: \textit{Type} }
    { Γ ⊢ \texttt{T}(C): \textit{Type} }

    \infer
    { Γ \text{ well-formed} }
    { Γ ⊢ \texttt{Bool}: \textit{BaseType} }

    \infer
    { Γ \text{ well-formed} }
    { Γ ⊢ \intty: \textit{BaseType} }

    \infer
    { Γ \text{ well-formed} }
    { Γ ⊢ \texttt{String}: \textit{BaseType} }

    \infer
    { Γ ⊢ A: \textit{BaseType} }
    { Γ ⊢ A: \textit{Type} }

    \infer
    { Γ, \alpha:K ⊢ A: \textit{Type} \\ \alpha \notin \textit{Dom}(Γ) }
    { Γ ⊢ \forall \alpha:K.A : \textit{Type} }

    \infer
    { Γ ⊢ A : \textit{Type} \\ Γ ⊢ B : \textit{Type} }
    { Γ ⊢ A \rightarrow B : \textit{Type} }

    \infer
    { Γ ⊢ A : \textit{Type} }
    { Γ ⊢ \texttt{List}\ A : \textit{Type} }

    \infer
    { Γ ⊢ R : \textit{Row} }
    { Γ ⊢ \texttt{Record}\ R : \textit{Type} }

    \infer
    { Γ ⊢ A : \textit{BaseType} }
    { Γ ⊢ \texttt{Trace}\ A : \textit{Type} }

    \infer
    { Γ ⊢ S: \textit{Row} }
    { Γ ⊢ \texttt{T}(S) : \textit{Row}}

    \infer
    { Γ \text{ well-formed} }
    { Γ ⊢ \cdot : \textit{Row} }

    \infer
    { Γ ⊢ A : \textit{Type} \\ Γ ⊢ R : \textit{Row} }
    { Γ ⊢ l:A;R : \textit{Row}}
  \end{mathpar}
  \caption{Type and row type kinding.}%formation $Γ ⊢ A : K$.}
  \label{fig:type-formation}
\end{figure}

Figure~\ref{fig:well-formed-contexts} defines well-formed, unified contexts $\Gamma$ as partial maps from term variables to types and from type variables to kinds.
Figure~\ref{fig:constructor-formation} shows the kinding rules for constructors and rows of constructors.
Similarly, Figure~\ref{fig:type-formation} shows the kinding rules for types and row types.
Morally, \textit{BaseType} is a subkind of \textit{Type} and \textit{BaseRow}, a row of base types, is a subkind of \textit{Row}.
We leave the subkinding relation implicit and mostly just use \textit{BaseType} as a hint, like in the kinding rule for \lstinline|Trace$^*$|.

\begin{figure}
  \footnotesize
  \begin{align*}
    S \leadsto S' \Rightarrow l:C; S &\leadsto l:C; S' \\
    C \leadsto C' \Rightarrow l:C; S &\leadsto l:C'; S \\
    \\
    C \leadsto C' \Rightarrow C\ D &\leadsto C'\ D \\
    D \leadsto D' \Rightarrow C\ D &\leadsto C\ D' \\
    (\lambda\alpha:K.C)\ D & \leadsto C[\alpha \coloneqq D] \\
    \\
    C \leadsto C' \Rightarrow \lambda \alpha:K.C &\leadsto \lambda \alpha:K.C' \\
    C \leadsto C' \Rightarrow \mathtt{List}^*\ C &\leadsto \mathtt{List}^*\ C' \\
    C \leadsto C' \Rightarrow \mathtt{Trace}^*\ C &\leadsto \mathtt{Trace}^*\ C' \\
    S \leadsto S' \Rightarrow \mathtt{Record}^*\ S &\leadsto \mathtt{Record}^*\ S' \\
    \\
    \kw{Rmap}\ C\ \cdot & \leadsto \cdot \\
    \kw{Rmap}\ C\ (l:D; S) &\leadsto (l: C\ D; \kw{Rmap}\ C\ S)\\
    S \leadsto S' \Rightarrow \kw{Rmap}\ C\ S &\leadsto \kw{Rmap}\ C\ S' \\
    C \leadsto C' \Rightarrow \kw{Rmap}\ C\ S &\leadsto \kw{Rmap}\ C'\ S \\
    \\
    C \leadsto C' \Rightarrow \kw{Typerec}~C~(C_B, C_I, C_S, C_L, C_R, C_T) &\leadsto \kw{Typerec}~C'~(C_B, C_I, C_S, C_L, C_R, C_T) \\
    C_B \leadsto C_B' \Rightarrow \kw{Typerec}~C~(C_B, C_I, C_S, C_L, C_R, C_T) &\leadsto \kw{Typerec}~C~(C_B', C_I, C_S, C_L, C_R, C_T) \\
    & \vdots \\
    \kw{Typerec}~\texttt{Bool}^*~(C_B, C_I, C_S, C_L, C_R, C_T) &\leadsto C_B \\
    \kw{Typerec}~\inttyc~(C_B, C_I, C_S, C_L, C_R, C_T) &\leadsto C_I \\
    \kw{Typerec}~\texttt{String}^*~(C_B, C_I, C_S, C_L, C_R, C_T) &\leadsto C_S \\
    \kw{Typerec}~\texttt{List}^*~D~(C_B, C_I, C_S, C_L, C_R, C_T) &\leadsto C_L\ D\ (\kw{Typerec}~D~(C_B, C_I, C_S, C_L, C_R, C_T)) \\
    \kw{Typerec}~\texttt{Record}^*~S~(C_B, C_I, C_S, C_L, C_R, C_T) &\leadsto C_R\ S\ (\kw{Rmap}\ (\lambda \alpha.\kw{Typerec}~\alpha~(C_B, C_I, C_S, C_L, C_R, C_T))\ S) \\
    \kw{Typerec}~\texttt{Trace}^*~D~(C_B, C_I, C_S, C_L, C_R, C_T) &\leadsto C_T\ D\ (\kw{Typerec}~D~(C_B, C_I, C_S, C_L, C_R, C_T))
  \end{align*}

  \caption{Constructor and row constructor computation.}
  \label{fig:constructor-computation}
\end{figure}

\begin{figure}
  \footnotesize
  \begin{mathpar}
    \infer
    { Γ ⊢ C : K }
    { Γ ⊢ C = C : K }

    \infer
    { Γ ⊢ D = C : K }
    { Γ ⊢ C = D : K }

    \infer
    { Γ ⊢ C = C' : K \\ Γ ⊢ C' = C'' : K }
    { Γ ⊢ C = C'' : K }

    \infer %some eta rule -- not really sure when this is needed
    { Γ ⊢ C : K \rightarrow K' }
    { Γ ⊢ \lambda\alpha:K.C\ \alpha = C: K \rightarrow K' }

    \infer
    { Γ,\alpha:K ⊢ C = D: K' \\ \alpha \notin \textit{Dom}(Γ) }
    { Γ ⊢ \lambda\alpha:K.C = \lambda\alpha:K.D: K \rightarrow K' }

    \infer
    { Γ ⊢ C = C' : K' \rightarrow K \\ Γ ⊢ D = D' : K' }
    { Γ ⊢ C\ D = C'\ D' : K }

    \infer
    { Γ ⊢ C = D : K }
    { Γ ⊢ \texttt{List}^*\ C = \texttt{List}^*\ D : K }

    \infer
    { Γ ⊢ S = S' : K }
    { Γ ⊢ \texttt{Record}^*\ S = \texttt{Record}^*\ S' : K }

    \infer
    { Γ ⊢ C = D : K }
    { Γ ⊢ \texttt{Trace}^*\ C = \texttt{Trace}^*\ D : K }

    \infer
    { Γ ⊢ C : K \\ Γ ⊢ D : K \\ C \leadsto D }
    { Γ ⊢ C = D : K }

    \infer
    { Γ \text{ well-formed} }
    { Γ ⊢ \cdot = \cdot : \textit{Row} }

    \infer
    { Γ ⊢ C = D: \textit{Type} \\ Γ ⊢ S = S': \textit{Row} }
    { Γ ⊢ (l:C; S) = (l:D; S') : \textit{Row} }

    \infer
    { Γ ⊢ C = D : \textit{Type} \rightarrow \textit{Type} \\ Γ ⊢ S = S' : \textit{Row} }
    { Γ ⊢ \kw{Rmap}\ C\ S = \kw{Rmap}\ D\ S' : \textit{Row} }

    \infer
    { Γ ⊢ C = C' : K \\
      Γ ⊢ C_B = C_B' : K \\
      Γ ⊢ C_I = C_I' : K \\
      Γ ⊢ C_S = C_S' : K \\
      Γ ⊢ C_L = C_L' : \textit{Type} \rightarrow K \rightarrow K \\
      Γ ⊢ C_R = C_R' : \textit{Row} \rightarrow \textit{Row} \rightarrow K \\
      Γ ⊢ C_T = C_T' : \textit{BaseType} \rightarrow K \rightarrow K }
    { Γ ⊢ \kw{Typerec}~C~(C_B, C_I, C_S, C_L, C_R, C_T) = \kw{Typerec}~C'~(C_B', C_I', C_S', C_L', C_R', C_T') : K }
  \end{mathpar}
  \caption{Constructor and row constructor equivalence.}% $Γ ⊢ C = D : K$ and row constructor equivalence $Γ ⊢ S = S' : K$.}
  \label{fig:constructor-equivalence}
\end{figure}

Constructors are equivalent according the rules in Figure~\ref{fig:constructor-equivalence} with type-level computation defined by the rules in Figure~\ref{fig:constructor-computation}.
Type-level computations include application of type-level functions, mapping of type-level functions over rows using \lstinline{Rmap}, and folding over types using \lstinline{Typerec}.
The rules do not enforce any particular evaluation order and may reduce nondeterministically anywhere inside a term.
Note also that type equality is symmetric so we can go, for example, from $\alpha$ to $(\lambda \alpha.\alpha)\ \alpha$ by symmetry and the type application $\beta$-rule.

\begin{figure}
  \footnotesize
  \begin{mathpar}
    \infer
    { Γ \text{ well-formed} }
    { Γ ⊢ \texttt{T}(\texttt{Bool}^*) = \texttt{Bool} : \textit{BaseType} }

    \infer
    { Γ \text{ well-formed} }
    { Γ ⊢ \texttt{T}(\inttyc) = \intty : \textit{BaseType} }

    \infer
    { Γ \text{ well-formed} }
    { Γ ⊢ \texttt{T}(\texttt{String}^*) = \texttt{String} : \textit{BaseType} }

    \infer
    { Γ ⊢ C : \textit{Type}}
    { Γ ⊢ \texttt{T}(\texttt{List}^*\ C) = \texttt{List}\ \texttt{T}(C) : \textit{Type} }

    \infer
    { Γ ⊢ S: \textit{Row} }
    { Γ ⊢ \texttt{T}(\texttt{Record}^*\ S) = \texttt{Record}\ \texttt{T}(S) : \textit{Type} }

    \infer
    { Γ ⊢ C : \textit{BaseType} }
    { Γ ⊢ \texttt{T}(\texttt{Trace}^*\ C) = \texttt{Trace}\ \texttt{T}(C) : \textit{Type} }

    \infer
    {  }
    { Γ ⊢ T(\cdot) = \cdot : \textit{Row} }

    \infer
    { Γ ⊢ C : \textit{Type} \\ Γ ⊢ S: \textit{Row} }
    { Γ ⊢ T(l:C; S) = (l:T(C); T(S)) : \textit{Row} }

    \infer
    { Γ ⊢ C = D : \textit{Type} }
    { Γ ⊢ \texttt{T}(C) = \texttt{T}(D) : \textit{Type} }

    \infer
    { Γ ⊢ S = S' : \textit{Row} }
    { Γ ⊢ \texttt{T}(S) = \texttt{T}(S') : \textit{Row} }

    \infer
    { Γ ⊢ A = B : \textit{Type}}
    { Γ ⊢ \texttt{List}\ A = \texttt{List}\ B: \textit{Type} }

    \infer
    { Γ ⊢ R = R' : \textit{Row} }
    { Γ ⊢ \texttt{Record}\ R = \texttt{Record}\ R' : \textit{Type} }

    \infer
    { Γ ⊢ A = B : \textit{BaseType} }
    { Γ ⊢ \texttt{Trace}\ A = \texttt{Trace}\ B : \textit{Type} }

    \infer
    { Γ ⊢ A = A' : \textit{Type} \\ Γ ⊢ B = B' : \textit{Type} }
    { Γ ⊢ A \rightarrow B = A' \rightarrow B' : \textit{Type} }

    \infer
    { Γ ⊢ A = B : \textit{Type}}
    { Γ ⊢ \forall \alpha. A = \forall \alpha. B : \textit{Type} }

    \infer
    { Γ \text{ well-formed} }
    { Γ ⊢ \cdot = \cdot : \textit{Row} }

    \infer
    { Γ ⊢ A = B: \textit{Type} \\ Γ ⊢ R = R': \textit{Row} }
    { Γ ⊢ (l:A; R) = (l:B; R') : \textit{Row} }

  \end{mathpar}
  \caption{Type and row type equivalence.}% $Γ ⊢ A = B: \mathit{Type}$.}
  \label{fig:type-equivalence}
\end{figure}

% \begin{figure}
%   \footnotesize
%   \begin{mathpar}
%     \infer
%     { Γ \text{ well-formed} }
%     { Γ ⊢ \cdot = \cdot : \textit{Row} }

%     \infer
%     { Γ ⊢ A = B: \textit{Type} \\ Γ ⊢ R = R': \textit{Row} }
%     { Γ ⊢ (l:A; R) = (l:B; R') : \textit{Row} }
%   \end{mathpar}
%   \caption{Row type equivalence $Γ ⊢ R = R' : \mathit{Row}$.}
%   \label{fig:row-type-equivalence}
% \end{figure}

Type equivalence is defined by the rules in Figure~\ref{fig:type-equivalence}.
There is no type-level computation in types, it all happens in constructors, but the equivalence rules for type \lstinline{T($C$)} show that the results of type-level computations have equivalents in types.
Note how unfinished type-level computations, in particular all the left-hand sides in Figure~\ref{fig:constructor-computation}, and type-level computations stuck on type variables are not equivalent to any type.

\begin{figure}
  \footnotesize
  \begin{mathpar}
    \infer
    { \Sigma(c) = A }
    { Γ ⊢ c : A}

    \infer
    { Γ(x) = A }
    { Γ ⊢ x : A}

    \infer
    { Γ ⊢ A : \textit{Type} \\
      Γ, x : A ⊢ M: B \\ x \notin \textit{Dom}(Γ)}
    { Γ ⊢ \lambda x:A.M : A \rightarrow B }

    \infer
    { Γ ⊢ M : A \rightarrow B \\ Γ ⊢ N : A }
    { Γ ⊢ M\ N : B }

    \infer
    { Γ,\alpha: K ⊢ M: A \\ \alpha \notin \textit{Dom}(Γ) }
    { Γ ⊢ \Lambda \alpha: K.M: \forall \alpha:K.A }

    \infer
    { Γ ⊢ M: \forall \alpha:K.A \\ Γ ⊢ C: K}
    { Γ ⊢ M\ C : A[\alpha \coloneqq C]}

    \infer
    { Γ ⊢ A \\ Γ,f:A ⊢ M:A}
    { Γ ⊢ \kw{fix}~f:A.M : A }

    \infer
    { Γ ⊢ L : \texttt{Bool} \\
      Γ ⊢ M : A \\
      Γ ⊢ N : A }
    { Γ ⊢ \kw{if}~L~\kw{then}~M~\kw{else}~N : A }

    \infer
    {Γ ⊢ M : \intty \\ Γ ⊢ N : \intty }
    {Γ ⊢ M + N : \intty }

    \infer
    {Γ ⊢ M : A \\ Γ ⊢ N : A \\ Γ ⊢ A : \textit{BaseType} }
    {Γ ⊢ M == N : \texttt{Bool} }

    \infer
    { \cdot ⊢ R : \textit{BaseRow} }
    {Γ ⊢ \kw{table}~n~\langle \textsf{oid}:\intty, R \rangle : \texttt{List} \langle \textsf{oid}:\intty; R \rangle}

    \infer % do I need an annotation ([]:A) and check that A is well-formed?
    { Γ ⊢ A: \textit{Type} }
    { Γ ⊢ [] : \texttt{List}\ A }

    \infer
    { Γ ⊢ M : A }
    { Γ ⊢ [M] : \texttt{List}\ A }

    \infer
    { Γ ⊢ M : \texttt{List}\ A \\ Γ ⊢ N : \texttt{List}\ A }
    { Γ ⊢ M \concat N  : \texttt{List}\ A }

    \infer % do we need Γ ⊢ A (like other binders: lambda, fix?) % annotate x? (x: A <- M)
    { Γ ⊢ M : \texttt{List}\ A \\ Γ,x:A ⊢ N : \texttt{List}\ B }
    { Γ ⊢ \kw{for}~(x \leftarrow M)~N : \texttt{List}\ B }

    \infer
    { Γ \text{ well-formed} }
    { Γ ⊢ \langle \rangle : \texttt{Record}\ ()}

    \infer
    { Γ ⊢ M : A \\ Γ ⊢ N : \texttt{Record}\ R }
    { Γ ⊢ \langle l = M; N \rangle : \texttt{Record}\ (l : A; R)}

    \infer
    { Γ ⊢ M : \texttt{Record}\ (l : A; R) }
    { Γ ⊢ M.l : A }

    \infer
    { Γ ⊢ M : B \\ Γ ⊢ A = B }
    { Γ ⊢ M : A }

    \infer
    { Γ ⊢ M : \forall \alpha: \textit{Type}. \texttt{T}(\alpha) \rightarrow \texttt{T}(C\ \alpha) \\
      Γ ⊢ N : \texttt{T}(\texttt{Record}^*\ S)}
    { Γ ⊢ \kw{rmap}^S~M~N : \texttt{T}(\texttt{Record}^*\ (\kw{Rmap}\ C \ S))}

    \infer
    { Γ ⊢ L: \texttt{T}(C) \rightarrow \texttt{T}(C) \rightarrow \texttt{T}(C) \\
      Γ ⊢ M : \texttt{T}(C) \\
      Γ ⊢ N : \texttt{T}(\texttt{Record}^*\ (\kw{Rmap}\ (\lambda\alpha.\alpha \rightarrow C)\ S)) }
    { Γ ⊢ \kw{rfold}^S\ L\ M\ N:\texttt{T}(C) }

    \infer
    { Γ ⊢ C : \textit{Type} \\
      Γ, \alpha: \textit{Type} ⊢ B : \textit{Type} \\
      \beta, \rho, \gamma \notin \textit{Dom}(Γ) \\
      Γ ⊢ M_B : B[\alpha \coloneqq \texttt{Bool}^*] \\
      Γ ⊢ M_I : B[\alpha \coloneqq \inttyc] \\
      Γ ⊢ M_S : B[\alpha \coloneqq \texttt{String}^*] \\
      Γ, \beta : \textit{Type} ⊢ M_L : B[\alpha \coloneqq \texttt{List}^*\ \beta] \\
      Γ, \rho : \textit{Row} ⊢ M_R : B[\alpha \coloneqq \texttt{Record}^*\ \rho] \\
      Γ, \gamma : \textit{BaseType} ⊢ M_T : B[\alpha \coloneqq \texttt{Trace}^*\ \gamma]
    }
    { Γ ⊢ \kw{typecase}~C~\kw{of}\ (M_B, M_I, M_S, \beta.M_L, \rho.M_R, \gamma.M_T) : B[\alpha \coloneqq C] }
  \end{mathpar}
  \caption{Term formation $Γ ⊢ M : A$.}
  \label{fig:term-formation}
\end{figure}

\begin{figure}
  \footnotesize
  \begin{mathpar}
    \infer
    { Γ ⊢ c : \texttt{Bool} }
    { Γ ⊢ \texttt{Lit}\ c : \texttt{Trace}\ \texttt{Bool} }

    \infer
    { Γ ⊢ c : \intty }
    { Γ ⊢ \texttt{Lit}\ c : \texttt{Trace}\ \intty }

    \infer
    { Γ ⊢ c : \texttt{String} }
    { Γ ⊢ \texttt{Lit}\ c : \texttt{Trace}\ \texttt{String} }

    \infer
    { Γ ⊢ M : \langle \mathsf{cond} : \texttt{Trace}\ \texttt{Bool}, \mathsf{out} : \texttt{Trace}\ A \rangle  }
    { Γ ⊢ \texttt{If}\ M : \texttt{Trace}\ A }

    \infer
    { Γ ⊢ C : \textit{Type} \\ Γ ⊢ M : \langle \mathsf{in} : \texttt{T(TRACE}\ C\texttt{)}, \mathsf{out} : \texttt{Trace}\ A \rangle  }
    { Γ ⊢ \texttt{For}\ C\ M : \texttt{Trace}\ A }

    \infer
    { Γ ⊢ M : \langle \mathsf{table} : \texttt{String}, \mathsf{column} : \texttt{String}, \mathsf{row} : \intty, \mathsf{data} : A \rangle  }
    { Γ ⊢ \texttt{Cell}\ M : \texttt{Trace}\ A }

    \infer
    { Γ ⊢ C : \textit{BaseType} \\ Γ ⊢ M : \langle \mathsf{left} : \texttt{T(TRACE}\ C\texttt{)}, \mathsf{right} : \texttt{T(TRACE}\ C\texttt{)} \rangle}
    { Γ ⊢ \texttt{OpEq}\ C\ M : \texttt{Trace}\ \texttt{Bool} }

    \infer
    { Γ ⊢ M : \langle \mathsf{left} : \texttt{Trace Int}, \mathsf{right} : \texttt{Trace Int}\rangle}
    { Γ ⊢ \texttt{OpPlus}\ M : \texttt{Trace}\ \intty }

    \infer
    { Γ ⊢ M : \texttt{Trace}\ A \\
      Γ, x_L : A ⊢ M_L : B \\
      Γ, x_I : \langle\mathsf{cond}: \texttt{Trace}\ \texttt{Bool}, \mathsf{then}: \texttt{Trace}\ A\rangle ⊢ M_I : B \\
      Γ, \alpha_F: \textit{Type}, x_F : \langle\mathsf{in}: \texttt{T}(\texttt{TRACE}\ \alpha_F), \mathsf{out}: \texttt{Trace}\ A\rangle ⊢ M_F : B \\
      Γ, x_C : \langle\mathsf{table}: \texttt{String}, \mathsf{column}: \texttt{String}, \mathsf{row}: \intty, \mathsf{data} : A\rangle ⊢ M_C : B \\
      Γ, \alpha_E : \textit{BaseType}, x_E : \langle\mathsf{left}: \texttt{T}(\texttt{TRACE}\ \alpha_E), \mathsf{right}: \texttt{T}(\texttt{TRACE}\ \alpha_E)\rangle ⊢ M_E : B \\
      Γ, x_P : \langle\mathsf{left}: \texttt{Trace}\ \intty, \mathsf{right}: \texttt{Trace}\ \intty\rangle ⊢ M_P : B \\
    }
    { Γ ⊢ \kw{tracecase}~M~\kw{of}\ (x_L.M_L, x_I.M_I, \alpha_F.x_F.M_F, x_C.M_C, \alpha_E.x_E.M_E, x_P.M_P) : B }
  \end{mathpar}

  \caption{\texttt{Trace} introduction and elimination rules.}
  \label{fig:trace-intro}
\end{figure}

The typing rules for terms are listed in Figure~\ref{fig:term-formation}.
We assume a signature $\Sigma$ that contains the types of constants $c$.
Unlike in \Links, we do not treat primitive operators like \lstinline|+| as constants.
We list explicit typing rules for \lstinline|+| and \lstinline|==| as representative examples (one monomorphic, one polymorphic) of the other arithmetic and relational operators.
The rule for tables enforces that every table has an \lstinline|oid| column.
There is no separate type for tables, instead tables just have an appropriate list type.
Unlike in \Links, we do not distinguish comprehensions over tables and lists syntactically.
The typing rules for \lstinline|rmap| and \lstinline|rfold| enforce that the annotated row constructor $S$ matches the record type.
The record fold rule additionally enforces that the record is homogeneous by requiring an \lstinline|Rmap| type with a constant function.

The typing rules for \lstinline|Trace| introduction and elimination in Figure~\ref{fig:trace-intro} make use of the type-level function \lstinline|TRACE| as defined in Figure \ref{fig:tracetf}.
The \lstinline|TRACE| function takes any query type and replaces all base types by their traced version.
We list rules for the operators \lstinline|+| and \lstinline|==| only.
\lstinline|OpPlus| serves as an example for the other monomorphic operators.
\lstinline|OpEq| similarly serves as an example for the other polymorphic operators.

Type-checking of \lamiml is decidable \citep{morrisett1995compiling,crary_weirich_morrisett_2002}.
We believe type-checking of \TLinks is decide-able, too.
Type inference is an issue.
\Urweb has generic record programming features that make type inference undesirably in general, but \citet{PLDI2010Chlipala} claims their heuristics make it still usable in practice.
Maybe something similar would work for \TLinks.

% \stefan{how much work would it be to actually prove that?}
% \james{I don't see any major obstacles.  The main issue is ensuring normalization of type constructors, which should go roughly the same way as normalization for System T, the only unusual thing is Rmap and the way Typerec uses Rmap for records.  But this all seems well-founded.  It would be good to nail this down in the (hopefully) eventual paper...}

% Type inference is an open question.
% \Urweb \cite{PLDI2010Chlipala} has generic record programming features that make type inference undecideable in general, but they claim their heuristics make it still useable in practice.

% \stefan{Third, related work / alternatives / whatnot}

% \stefan{this is likely not the only possible solution. \textsc{gadt}s allow doing similar things (maybe with type families and datafamilies?), but typerec seems like the smaller extension to a \Links-like language where \textsc{adt}s are encoded as recursive variants.}

% \stefan{According to \cite{crary_weirich_morrisett_2002}, type-checking of $\lambda_i^\mathit{ML}$ is decidable.
% Type inference is an open question.
% \Urweb has generic record programming features that make type inference undecideable in general, but they claim their heuristics make it still useable in practice.
% While we aim for users being able to implement their own forms of provenance by writing trace analysis functions, it is certainly an advanced feature and we can tolerate having to write type annotations.}

\section{Recovering provenance from traces}\label{sec:trace-analyses}

In this section we demonstrate how to use \TLinks to write trace analysis functions that extract provenance from traces.
We start with the \lstinline|value| function, which extracts the plain, unannotated value from a trace, then move on to where-provenance (Section~\ref{sec:taf-where}) and lineage (Section~\ref{sec:taf-lineage}).

\subsection{Value}
\label{sec:taf-value}
% \epigraph{Eventually I came to regard nondeterminacy as the normal situation, determinacy being reduced to a —not even very interesting— special case.}{E. W. Dijkstra \\[-0.5em] {\scriptsize A Discipline of Programming, 1976, page xv}}

% \noindent
The purpose of tracing queries is to extract provenance.
However, we can use the same mechanism to extract the original values from a trace.
% \citet{misinterpretingsql} call it \emph{what}-provenance
Basically, applying the \lstinline|value| trace analysis function to the trace of a query $Q$ should have the same result as $Q$ itself without any tracing.

On the level of types we have that tracing a query $Q$ of type $C$ results in a trace of type \lstinline|TRACE $C$|.
The type-level function \lstinline|VALUE| in Figure~\ref{fig:value} undoes what \lstinline|TRACE| does.
On base types it is the identity; on list and record types it recursively applies itself to element and field types; and on trace types it removes the type constructor \lstinline|Trace|.
In other words \lstinline|VALUE| is the left inverse of \lstinline|TRACE| on nested relational query types.
\begin{lemma}\label{lem:valuetf-inverse}
  For all query type constructors $C$ and row constructors $S$ and well-formed contexts $\Gamma$:
  \[ \Gamma \vdash \mathtt{VALUE}(\mathtt{TRACE}\ C) = C \] and
  \[ \Gamma \vdash \kw{Rmap}\ \mathtt{VALUE}\ (\kw{Rmap}\ \mathtt{TRACE}\ S) = S \]
\end{lemma}

% \james{Would it work to define "value" at type forall a. T(TRACE a) -> T(a) ?} \stefan{Uh. maybe?}

\begin{figure}
\begin{lstlisting}
VALUE = $\lambda$a:Type.Typerec a (Bool, Int, String,
                  $\lambda$_ b.List b, $\lambda$_ r.Record r, $\lambda$c _.c)

value : $\forall$a.T(a) -> T(VALUE a)
value = fix (value: $\forall$a.T(a) -> T(VALUE a)).$\Lambda$a:Type.
  typecase a of
    Bool     => $\lambda$x:Bool.x
    Int      => $\lambda$x:Int.x
    String   => $\lambda$x:String.x
    List b   => $\lambda$x:List b.for (y <- x) [value b y]
    Record r => $\lambda$x:Record r.rmap$^\texttt{r}$ value x
    Trace b  => $\lambda$x:Trace b.tracecase x of
      Lit y    => y
      If y     => value (Trace b) y.out
      For c y  => value (Trace b) y.out
      Cell y   => y.data
      OpPlus y => value (Trace Int) y.left +
                  value (Trace Int) y.right
      OpEq c y => value (TRACE c) y.left ==
                  value (TRACE c) y.right
\end{lstlisting}
  \caption{The \texttt{value} trace analysis function and \texttt{VALUE} type-level function.}
  \label{fig:value}
\end{figure}

The \lstinline|value| function is shown in Figure \ref{fig:value}.
It has the polymorphic type \lstinline|$\forall$a.a -> VALUE a|.
Thus, when we apply it to the type \lstinline|TRACE $C$| we get a function from \lstinline|TRACE $C$| to \lstinline|VALUE (TRACE $C$)| which is the same as $C$, exactly as expected.

The implementation of \lstinline|value| is by \lstinline|typecase|.
For the base types nothing needs to be done and \lstinline|value| behaves like the identity.
In fact, when \lstinline|value| is applied to a trace generated by \TLinks, these cases will never be encountered.
To obtain a list of values from a list of $b$s we traverse the list using a \lstinline|for| comprehension and recursively call the \lstinline|value| function at the element type \lstinline|b|.
Similarly for records we map the \lstinline|value| function over the record fields.
This is where the first of the generic record programming features of \TLinks comes in.
The new keyword \lstinline|rmap| calls \lstinline|value| with the type and value of every field in the record~\lstinline|x| and collects the result in a new record.
Upon reaching an actual trace we case-split on the constructor using \lstinline|tracecase|.
Literals carry their value directly.
\lstinline|If| and \lstinline|For| nodes both carry a subtrace of the same type so we recursively call \lstinline|value| on that.
A database \lstinline|Cell| carries its value in the \lstinline|data| field.
Finally, the various operator traces carry subtraces on which we recursively call \lstinline|value| and then combine the results using the appropriate operator.

The \lstinline|value| function is structurally recursive.

\subsection{Where-provenance}\label{sec:taf-where}

This section describes how to extract where-provenance from a trace.
With \WLinks we explored type system extensions to make handling where-provenance safer and give static guarantees about the presence of useful annotations.
Here we use a more traditional approach in which where-provenance annotations are just more data, like lineage in \LLinks.

We replace every cell in the output with a record of the original data as well as table, column, and row number.
On the type-level this is done by \lstinline|WHERE| defined in Figure \ref{fig:where-ta}.
Base types in the result are replaced by record types using the helper function \lstinline|W|.
Like in \lstinline|VALUE| before, lists and records are just traversed recursively.
Traces are replaced by \lstinline|W|.
For example:
\begin{lstlisting}
  WHERE (TRACE [{a: Int, b: [String]}])
= WHERE [{a: Trace Int, b: [Trace String]}]
= [{a: W Int, b: [W String]}]
= [{a: {data: Int, %table%:String, column:String, row:Int},
    b: [{data: String, %table%:String, column:String, row:Int}]}]
\end{lstlisting}

\begin{figure}
\begin{lstlisting}[literate={{/}{{/}}{1}{\{}{{$\langle$}}{1}{\}}{{$\rangle$}}{1}}]
W = $\lambda$a:Type.{data:a, %table%:String, column:String, row:Int}

WHERE = $\lambda$a:Type.Typerec a (W Bool, W Int, W String,
                  $\lambda$_ b.List b, $\lambda$_ r.Record r, $\lambda$_ b.b)

wherep : $\forall$a.T(TRACE a) -> T(WHERE a)
wherep = fix (wherep:$\forall$a.T(TRACE a) -> T(WHERE a)).$\Lambda$a:Type.
  typecase a of
    Bool     => fake Bool
    Int      => fake Int
    String   => fake String
    List b   => $\lambda$xs.for (x <- xs) [wherep b x]
    Record r => $\lambda$x.rmap$^\texttt{r}$ wherep x
    Trace b  => $\lambda$x.tracecase x of
      Lit y    => fake b y
      If y     => wherep (Trace b) y.out
      For c y  => wherep (Trace b) y.out
      Cell y   => y
      OpPlus y => fake Int (value (Trace Int) y.left +
                            value (Trace Int) y.right)
      OpEq c y => fake Bool (value (TRACE c) y.left ==
                             value (TRACE c) y.right)

fake : $\forall$a.T(a) -> T(W a)
fake = $\Lambda$a:Type.$\lambda$x:T(a).{data = x, %table% = "facts",
                        column = "alternative", row = -1}
\end{lstlisting}

  \caption{The \texttt{wherep} trace analysis function and supporting definitions.}
  \label{fig:where-ta}
\end{figure}

The trace analysis function \lstinline|wherep| itself is defined in Figure~\ref{fig:where-ta} and has type \lstinline|$\forall$a.T(TRACE a) -> T(WHERE a)|.
The overall structure is much the same as the \lstinline|value| function before:
we define a recursive, polymorphic function by cases on the argument type.
The base cases are unreachable because a trace will always have leaves of \lstinline|Trace| types, see Lemma~\ref{lem:trace-non-base}.
Therefore it does not matter what the implementation is, as long as it typechecks.
The helper function \lstinline|fake| annotates a value with a fake annotation---something like $\bot$.
For lists and records we map \lstinline|wherep| over the elements and fields, respectively.
Traces of literals are annotated with a fake annotation to indicate that they do not come from the database.
As before, the cases for \lstinline|If| and \lstinline|For| annotate their output.
The case for a database cell is the most important, yet trivial:
The \lstinline|Cell| trace constructor already carries value and where-provenance in exactly the right format, so we just return it.
Finally, the operators use the \lstinline|value| function to compute values from subtraces, perform the appropriate operation and annotate the result with a fake annotation.

This implementation demonstrates that it is possible to compute where-provenance using this tracing approach.
It is easy to see how we could use \TLinks to implement further variants of where-provenance at least as flexible as the limited user-defined annotations in \WLinks.
It is not at all clear how to recover the strong typing discipline for provenance annotations that \WLinks provides.

\subsection{Lineage}\label{sec:taf-lineage}

As far as possible, this implementation of lineage aims to emulate the behavior of \LLinks as described in Chapter \ref{cha:llinks}.
This is slightly challenging, because lineage annotations in \LLinks are on rows (or more generally, list elements) but tracing information in \TLinks is on cells.
We need to collect annotations from the leaves and pull them up to the nearest enclosing list constructor.

On the type-level, we have the \lstinline|LINEAGE| function as defined in Figure \ref{fig:lineage-ta}.
The purpose of \lstinline|LINEAGE| is the same as that of the lineage type translation $𝔏$ from Chapter~\ref{cha:llinks} defined in Figure~\ref{fig:llinks-type-translation}.
Given a query type it places an annotation on every list element type.
For example:
\begin{lstlisting}
  LINEAGE [{a: [Int]}]
= [L {a: [L Int]}]
= [{data: {a: [{data: Int,
                lineage: [{%table%: String, row: Int}]}]},
    lineage: [{%table%: String, row: Int}]}]
\end{lstlisting}

We have $\forall \alpha:\mathit{Type}. \texttt{LINEAGE}\ (\texttt{TRACE}\ \alpha) = \texttt{LINEAGE}\ \alpha$.
The only interesting case is the one for record types, where we apply the induction hypothesis on the composition of type functions in a row map operation on a smaller type $\rho$: $\kw{Rmap}\ (\texttt{LINEAGE}\cdot\texttt{TRACE})\ \rho = \kw{Rmap}\ \texttt{LINEAGE}\ \rho$.

\begin{figure}
\begin{lstlisting}
L = $\lambda$a:Type.{data: a, lineage: [{%table%: String, row: Int}}

LINEAGE = $\lambda$a:Type.Typerec a (Bool, Int, String,
                    $\lambda$_ b.List (L b), $\lambda$_ r.Record r, $\lambda$_ b.b)

lineage : $\forall$a.T(TRACE a) -> T(LINEAGE a)
lineage = fix (lineage:$\forall$a.T(TRACE a) -> T(LINEAGE a)).$\Lambda$a:Type.
  typecase a of
    Bool | Int | String => id a  -- unreachable
    List b   => $\lambda$ts.for (t <- ts)
                    [{data = lineage b t,
                      lineage = linnotation b t}]
    Record r => $\lambda$x.rmap$^\texttt{r}$ lineage x
    Trace b  => $\lambda$x.value (Trace b) x

linnotation : $\forall$a.T(TRACE a) -> [{%table%: String, row: Int}]
linnotation = fix (linnotation: ...).$\Lambda$a:Type.
  typecase a of
    Bool | Int | String => $\lambda$_.[]
    List b   => $\lambda$ts.for (t <- ts) linnotation b t
    Record r => $\lambda$x.rfold$^{\texttt{Rmap }(\lambda\texttt{\_.[}\langle\texttt{table:String, row:Int}\rangle\texttt{]})\texttt{ r}}$ (++) []
                      (rmap$^\texttt{r}$ linnotation x)
    Trace b  => $\lambda$t.tracecase t of
      Lit c    => []
      If i     => linnotation (TRACE b) i.out
      For c f  => linnotation (TRACE c) f.in ++
                  linnotation (TRACE b) f.out
      Cell r   => [{%table% = r.%table%, row = r.row}]
      OpEq c e => linnotation (TRACE c) e.left ++
                  linnotation (TRACE c) e.right
      OpPlus p => linnotation (TRACE Int) p.left ++
                  linnotation (TRACE Int) p.right
\end{lstlisting}

  \caption{The \texttt{lineage} trace analysis function and supporting definitions.}
  \label{fig:lineage-ta}
\end{figure}

On the value-level the implementation is split into two functions: \lstinline|lineage| and \lstinline|linnotation|, as shown in Figure~\ref{fig:lineage-ta}.
The \lstinline|lineage| function matches on the type of its argument and makes (recursive) calls to \lstinline|lineage|, \lstinline|linnotation|, and \lstinline|value| as appropriate.
The \lstinline|linnotation| function does the actual work of computing lineage annotations from traces.
It assigns an empty list of annotations to base types (again, these are unreachable for traced queries).
The case for lists concatenates the lineage annotations obtained by calling \lstinline|linnotation| on the list elements.
The case for records does the same, but in a slightly more roundabout way:
We first use \lstinline|rmap| to map \lstinline|linnotation| over the record, then we use \lstinline|rfold| to flatten the record of lists of lineage annotations into a single list.\footnote{
  The attentive reader might remember that we previously pointed out that it is best to use a commutative combining function in \lstinline|rfold| because record labels are unordered.
  Here we use list concatenation which is decidedly non-commutative.
  More on this in a bit.}
Trace constructors have lineage annotations as follows.
Literals do not have lineage.
Conditional expressions have the lineage of their result.
Comprehensions are the interesting case, where we combine lineage annotations from the input with lineage annotations from the output.
Each table cell has the expected initial singleton annotation consisting of its table's name and its row number.
Finally, the operators just collect their arguments' annotations.

There is an issue with this implementation of lineage: we collect duplicate annotations.
Consider the following query:
\begin{lstlisting}[literate={{/}{{/}}{1}{\{}{{$\langle$}}{1}{\}}{{$\rangle$}}{1}}]
for (x <- table "xs" {a: Int, b: Bool, c: String}) [x.a]
\end{lstlisting}
We just project a table to one of its columns.
The lineage of every element of the result should be one of the rows in the table.
If we apply the \lstinline|lineage| trace analysis function to the trace of the above query (at the appropriate type) and normalize, we get this query expression:
\begin{lstlisting}
for (x <- table "xs" {a: Int, b: Bool, c: String})
  [{data = x.a,
    lineage = [{%table% = "xs", row = x.oid}] ++
              [{%table% = "xs", row = x.oid}] ++
              [{%table% = "xs", row = x.oid}] ++
              [{%table% = "xs", row = x.oid}]}]
\end{lstlisting}
The lineage is correct, but there is too much of it.
Instead of having one annotation with table and row, we have the same annotation four times.
In fact, a similar query on a table with $n$ columns, would produce $n+1$ annotations.
Looking at the (normalized) traced expression below, we can see the problem.
\begin{lstlisting}
for (x <- table "xs" {a: Int, b: Bool, c: String})
  [For {in={a=Row {%table%="xs", column="a", row=x.oid, data=x.a},
            b=Row {%table%="xs", column="b", row=x.oid, data=x.b},
            c=Row {%table%="xs", column="c", row=x.oid, data=x.c}},
        out=Row {%table%="xs", column="a", row=x.oid, data=x.a}}]
\end{lstlisting}
The record case combines the annotations from all of the fields, which interacts badly with the tracing of tables, which puts annotations on all of the fields.
Our definition of lineage from Chapter \ref{cha:llinks} is really about rows, not cells.
This clashes with our traces, which are on cells, not rows.
There are at least two solutions to this problem that preserve tracing at the level of cells.
The ad-hoc solution is not optimal in general, but would be sufficient here, and maybe other cases:
We could introduce a set union operator $M \cup N$ with a special normalization rule that reduces to just $M$ if $M$ and $N$ are known to be equal statically, at query normalization time.
In the example above we would only need to test alpha equivalence, but other queries and other forms of provenance might require more sophisticated analysis for determining duplicates.
The proper solution would be to support set and multiset semantics for different portions of the same query and generate \SQL queries that eliminate duplicates where necessary.

\subsection{Other forms of provenance}

Following the same approach, it should be possible to implement other forms of provenance based on annotation propagation, such as the cell-level lineage of \citet{misinterpretingsql}.
Dependency provenance \citep{MSCS2011CheneyAA} has annotations on multiple levels which may be difficult to recover from cell-level traces alone.
Semiring provenance is another interesting candidate.
One challenge is, again, that it is defined on rows.
One opportunity is that trace analysis functions are just that, functions, so a generic semiring trace analysis function could be parameterized by concrete $+$ and $\times$ operations and $0$ and $1$ values.

Expression provenance \citep{10.1007/978-3-642-28641-4_22} annotates values with a tree of abstract expressions that were executed to obtain the value.
Conceptually this is very close to the trace itself but the \texttt{Trace} type is not a query type.
To implement expression provenance in \TLinks we would need to find a suitable (nested) relational encoding.
\citet{DDFP2013GiorgidzeGUW} show how to encode arbitrary nonrecursive algebraic datatypes relationally and use this in an extension to the language-integrated query library \DSH.
The datatype for expressions is recursive, but of a limited depth and thus can be unrolled.
It seems possible to do all of this in a trace analysis function, but perhaps it would be more fruitful to extend \TLinks itself to deal with algebraic datatypes to make this easier.
Unfortunately, even full support for recursive algebraic datatypes is not quite enough to define the \lstinline|Trace| type in the language, because that also needs to store type information for polymorphic operations and comprehensions.

% \james{Peter's high-level comments:\\
% 2) He also wanted to know why not consider other forms of provenance such as associating a small tree/graph with each annotated part of the data.  For example what is called "expression provenance" in the "core calculus for provenance" paper.  I think the answer may be "could do that, but it would be a hassle without some language support for algebraic datatypes in queries" - something that DSH supported at one point (at least non-recursive ones) but currently does not. \\
% Alternatively, I could imagine having the "annotations" be sets of triples representing some RDF data.  (I think Natalia Kwasnikowska proposed something like this in her thesis with Jan van den Bussche).  But here the problem would probably be coming up with unique identifiers for new graph nodes when needed.
% }

Combining forms of provenance is another interesting exercise.
We have already seen multiple trace analysis functions used together: both \lstinline|wherep| and \lstinline|lineage| use \lstinline|value|.
However, it would be ill-typed to call \lstinline|wherep| and then \lstinline|lineage| on a query trace, because \lstinline|wherep| does not preserve the trace.
Manually fusing the where-provenance and lineage analysis functions is certainly possible, but somewhat dissatisfying.
It would be interesting to see if they can be written in a way that preserves a copy of the trace, so that multiple trace analysis functions could be stacked.

Fortunately, it is not necessary to extend \TLinks to define new forms of provenance or provenance combinators, which should make it much easier to carry out such experiments in the future.

\section{Self-tracing queries}
\label{sec:self-tracing-queries}

This section describes the transformation that turns a normalized query $Q_n$ into a query $Q_t$ that, when executed, returns a trace of the execution of $Q_n$.

\begin{figure}
\begin{lstlisting}
TRACE = $\lambda$a. Typerec a (Trace Bool, Trace Int, Trace String,
                       $\lambda$ _ b. List b, $\lambda$ _ r. Record r, $\lambda$ _ b. b)
\end{lstlisting}
  \caption{The type-level function \lstinline!TRACE!.}
  \label{fig:tracetf}
\end{figure}

As mentioned before, the most important aspect of our notion of traces is that all the tracing information is at the level of base types.
An annotated value of base type $A$ has type \lstinline{Trace $A$}.
Records and lists on the other hand do not carry any annotations themselves.
In other words, the trace of a list is a list of traces and the trace of a record is a record of traces.
A query typically has a larger type than just a base type, at least a list constructor.
The type-level function \lstinline{TRACE}, defined in Figure~\ref{fig:tracetf}, describes the type of a traced query.
If a query $Q_n$ has type $C$, its traced version $Q_t$ has type \lstinline|TRACE C|.
\lstinline|TRACE| is defined in terms of \lstinline{Typerec} to recursively traverse a tree made of \lstinline{List} and \lstinline{Record} constructors and apply the \lstinline{Trace} type constructor to all the base types at the leaves of the tree.
For example:
\begin{lstlisting}
  TRACE [{a: [Int], b: {c: String}}]
= [TRACE {a: [Int], b: {c: String}}]
= [{a: TRACE [Int], b: TRACE {c: String}}]
= [{a: [TRACE Int], b: {c: TRACE String}}]
= [{a: [Trace Int], b: {c: Trace String}}]
\end{lstlisting}

\begin{lemma}\label{lem:trace-non-base}
  For all query types $C$, \lstinline|TRACE| $C$ is not a base type.
\end{lemma}

\begin{figure}[t]
  \footnotesize
  \begin{align*}
    \trace{x} &= x \\
    \trace{c} &= \texttt{Lit}\ c \\
    \ttrace{\kw{if}~L~\kw{then}~M~\kw{else}~N}{C}
              &= \kw{if}~\texttt{value (Trace Bool)}\ \trace{L}\\
              & \hspace{-4em} \kw{then}~ \mathit{dist}(\texttt{TRACE}\ C, \texttt{If}\ \langle \texttt{cond} = \trace{L}, \texttt{out} = \mathbb{H} \rangle)\ \trace{M} \\
              & \hspace{-4em} \kw{else}~ \mathit{dist}(\texttt{TRACE}\ C, \texttt{If}\ \langle \texttt{cond} = \trace{L}, \texttt{out} = \mathbb{H} \rangle)\ \trace{N} \\
    \trace{[]} &= [] \\
    \trace{[M]} &= [\trace{M}] \\
    \trace{M \concat N} &= \trace{M} \concat \trace{N} \\
    \ttrace{\kw{for}~(x \leftarrow M:D)~N}{C} &= \kw{for}~(x \leftarrow \trace{M})\\
              & \hspace{-4em} \mathit{dist}(\texttt{TRACE}\ C, \texttt{For}\ D\ \langle \texttt{in} = x, \texttt{out} = \mathbb{H} \rangle)\ \trace{N} \\
    \trace{\langle \overline{ l = M } \rangle} &= \langle \overline{l = \trace{M}}\rangle \\
    \trace{M.l} &= \trace{M}.l \\
    \trace{\kw{table}~n~\langle \overline{l : C} \rangle}
              & = \kw{for}\ (y \leftarrow \kw{table}~n~\langle \overline{l : C} \rangle) \\
              & \qquad [\langle\overline{l = \mathit{cell}(n, l, y.\texttt{oid}, y.l)}\rangle ] \\
    \trace{M == (N: \texttt{T}(C))} &= \texttt{OpEq}\ C\ \langle \texttt{left} = \trace{M}, \texttt{right} = \trace{N}\rangle \\
    \trace{M + N} &= \texttt{OpPlus}\ \langle \texttt{left} = \trace{M}, \texttt{right} = \trace{N}\rangle
  \end{align*}
  \begin{align*}
    \mathit{cell}(t,c,r,d) & = \texttt{Cell}\langle\texttt{table}=t,\texttt{column}=c,\texttt{row}=r,\texttt{data}=d\rangle \\
    \mathit{dist}(\langle \overline{l:C} \rangle, k) &= \lambda r:\langle \overline{l:C} \rangle.\langle \overline{ l = \mathit{dist}(C,k)\ (r.l) }\rangle \\
    \mathit{dist}(\texttt{Trace}\ C, k) &= \lambda t:\texttt{Trace}\ C.k[\mathbb{H} \coloneqq t]\\
    \mathit{dist}(\texttt{List}\ C, k) &= \lambda l:\texttt{List}\ C.\kw{for}\ (x \leftarrow l)\ [\mathit{dist}(C, k)\ x]
  \end{align*}
  \caption{Self-tracing transformation.}
  \label{fig:self-tracing}
\end{figure}

Figure~\ref{fig:self-tracing} shows the self-tracing transformation $\trace{\cdot}$ and two helper functions.
The self-tracing transformation takes a term of type \lstinline{T($C$)} and returns a self-tracing query of type \lstinline{T(TRACE $C$)} for any query type $C$.
The $\mathit{dist}$ function is a meta-level helper function that takes a type and an expression with a hole $\mathbb{H}$ in it.
It produces an object-level function that takes a value of the given type and traverses lists and records until it reaches all the leaves and wraps the expression with the hole around them.\footnote{We could write \textit{dist} as an object-level function with the type below, but going from what is basically a partially applied \lstinline{Trace} constructor to a fully polymorphic function involves a lot of boilerplate code for handling impossible non-base-type cases.\\\lstinline{dist: forall a. (forall b. Trace b -> Trace b) -> TRACE a -> TRACE a}}
It is used to push down trace information over list and record constructors and into the leaves.

We apply the tracing transformation to normalized queries.
We do not rely on the normal form itself, but only on the absence of non-primitive functions, variants, and free variables.
Thus, all variables that appear in a query are introduced by for-comprehensions.

Variables are left untouched by the transformation, but in the self-tracing query they have different types, namely trace types, as seen in the translation of for-comprehensions.
Literal values in the query are annotated with the \lstinline{Lit} constructor.
To trace if-then-else we need to trace both branches and return the correct one depending on whether the condition holds at runtime.
We use the trace analysis function \lstinline{value} (defined in Section~\ref{sec:taf-value}) to turn the trace of the condition, which has type \lstinline{Trace Bool}, back into a plain unannotated \lstinline{Bool}.
This simplest of the trace analysis functions discards all trace annotations and is described in more detail in Section~\ref{sec:taf-value}.
We cannot just \emph{not} trace the condition, because it may contain bound variables, but their type is different in the self-tracing query.
We use the $\mathit{dist}$ function to distribute an annotation over both branches that also contains the trace of the conditional.
The cases for empty lists, singleton lists, and list concatenation are the obvious ones considering that a trace of a list is a list of traces.
Self-tracing for-comprehensions iterate over traced input and annotate every output element with the corresponding input, again using $\mathit{dist}$.
Note that as mentioned before the variables bound by comprehensions have different types in the original and self-tracing query.
Record construction and projection are again the obvious translations considering that a trace of a record is a record of traces.
Tables are translated to iterations over the tables that provide initial annotations, similar to the where-provenance and lineage transformations earlier.
Here the initial annotation uses the $\mathit{cell}$ function which is just the \lstinline{Cell} constructor in disguise.
It takes the familiar annotations table name, column name, row number via \lstinline{oid}, and the data itself.
Operators like \lstinline{==} and \lstinline{+} record subtraces for their arguments.
Equality, as a polymorphic operation, additionally records the type at which it was applied.
We need this later when analyzing a trace.

As a sanity check we prove that the result of the tracing transformation is type correct.
We prove a lemma about $\mathit{dist}$ first.

\begin{lemma}[Distributing trace constructors is type correct]\label{lem:dist-type-correctness}
  For all types $C$ that can appear in query types (base types, list types, closed record types) and all expressions $k$ with a hole $\mathbb{H}$ that have type $\texttt{Trace}\ D$ assuming the hole $\mathbb{H}$ has type $\texttt{Trace}\ D$, $\mathit{dist}(\texttt{TRACE}\ C, k)$ has type $\texttt{TRACE}\ C \rightarrow \texttt{TRACE}\ C$.
  \begin{gather*}
    \forall \Gamma, C, k : \mathit{QueryType(C)} \wedge (\forall D: \mathit{BaseType(D)} \Rightarrow \Gamma, \mathbb{H}:\texttt{Trace}\ D \vdash k:\texttt{Trace}\ D) \\
    \Longrightarrow \quad \Gamma \vdash \mathit{dist}(\texttt{TRACE}\ C, k):\texttt{TRACE}\ C \rightarrow \texttt{TRACE}\ C
  \end{gather*}
\end{lemma}

We only trace closed terms.
However, we cannot require an empty context, because then the induction would not work out for comprehensions.
Therefore we define a tracing transformation on contexts as follows.
\begin{definition}[Trace context]\label{def:trace-context}
  $\trace{\Gamma}$ maps term variable $x$ to \lstinline|T(TRACE $C$)| if and only if $\Gamma$ maps $x$ to $A$, where $C$ is the obvious constructor with $\cdot \vdash A = \texttt{T}(C)$.
\end{definition}

\begin{lemma}\label{lem:nrc-types-constr}
  For every query type $A$ made of base types, list constructors, and closed records, there exists $C$ such that $\Gamma \vdash A = \mathtt{T}(C)$ in a well-formed context $\Gamma$.
\end{lemma}

% \james{Is it safe to restrict attention to NRC types $A$ from now?}
% \stefan{It mostly is, except that the theorem is about the TRACE type function, so it unfortunately really has to live in C.}

% \james{I think the real induction hypothesis should be something like
% if Gamma |- M : A
% then for all C. if A = T(C)
% then [[Gamma]] |- [[M]] : T(TRACE C)\\
% then any cases that derive types that cannot be of the form T(C) you can rule out, and all other cases you can say "let C be given such that A = T(C)" and proceed.\\
% (I'm not sure here whether you want an assumption that A = T(C) syntactically or a judgment Gamma |- A = T(C).  If the former works it's probably simpler.)}

\begin{theorem}[Trace rewriting is type correct]\label{thm:trace-type-correctness-2}
  If $\Gamma \vdash M : A$ then for all $C$,
  if $\Gamma \vdash A = \mathtt{T}(C)$
  then $\trace{\Gamma} \vdash \trace{M} : \mathtt{T}(\mathtt{TRACE}\ C)$,
  where $\Gamma$ is a context that maps all term variables to closed records with fields of base type
  and $M$ is a plain \Links query term in normal form.
\end{theorem}

\section{Normalization}\label{sec:tlinks-normalization}

Our ultimate goal is to translate \TLinks queries --- including provenance extraction by trace analysis --- to \SQL.
In Section \ref{sec:tlinks-redrel} we define the reduction relation~$\leadsto$ on \TLinks terms, constructors, and row constructors.
In Section \ref{sec:tlinks-preservation}, we show that this reduction relation preserves types.
Section \ref{sec:tlinks-normal-form} describes the \TLinks normal form.
In Section \ref{sec:tlinks-progress} we prove a progress lemma: well-typed terms reduce or are in \TLinks normal form.
This is slightly different from standard progress in that the normal form is not a \emph{value}.
Rather, the normal form describes partially evaluated programs that cannot reduce further, because they are stuck on either database table references, or free variables.
Progress and preservation imply the existence of a partial normalization function.
Section \ref{sec:tlinks-tighten} tightens the normal form for queries.
Closed terms with query type, if they normalize at all, normalize to a term in the nested relational calculus.
From there we can use previous work, for example query shredding \citep{SIGMOD2014CheneyLW} or flattening \citep{SIGMOD2015UlrichG}, to go the rest of the way to flat \SQL queries.

% \james{Might be worth pointing out the similarities and differences with "standard" progress/preservation:
% - reduction under lambda, inside comprehensions etc.
% - goal is not just to ensure lack of "stuckness" but that the normal forms are suitable input for later query compilation stages
% - we might also want to prove termination/strong normalization (subject to some caveat about recursion) but that would be a lot of effort for relatively little practical benefit.}

\subsection{Reduction relation}\label{sec:tlinks-redrel}

The reduction relation $\leadsto$ is overloaded for constructors, row constructors, and terms.
We have already seen the reduction rules for constructors and row constructors in Figure \ref{fig:constructor-computation}.
% Figure~\ref{fig:normalization-beta} lists the $\beta$-reduction rules for terms.
% There are additional congruence rules in Figure \ref{fig:normalization-rules-congruence}.
The reduction rules for terms are inspired by previous work on \Links query normalization \citep{DBPL2009Cooper,TLDI2012LindleyC,SIGMOD2014CheneyLW}.

\begin{figure*}
  \footnotesize
  \begin{align*}
    (\lambda x.M)\ N &\leadsto M[x \coloneqq N] \\
    \kw{fix}~f.M &\leadsto M[f \coloneqq \kw{fix}~f.M] \\
    (\Lambda \alpha.M)\ C &\leadsto M[\alpha \coloneqq C] \\
    \kw{if}~\kw{true}~\kw{then}~M~\kw{else}~N &\leadsto M \\
    \kw{if}~\kw{false}~\kw{then}~M~\kw{else}~N &\leadsto N \\
    \langle \overline{l_i=M_i}  \rangle.l_i &\leadsto M_i \\
    \kw{rmap}^{(\overline{l_i:C_i})}\ M\ N &\leadsto \langle \overline{l_i = (M\ C_i)\ N.l_i } \rangle \\
    \kw{rfold}^{(\overline{l_i: C_i})}\ L\ M\ N & \leadsto L\ N.l_1\ (L\ N.l_2 \hdots (L\ N.l_n\ M) \hdots) \\
    \kw{for}~(x \leftarrow [])~N &\leadsto [] \\
    \kw{for}~(x \leftarrow [M])~N &\leadsto N[x \coloneqq M]
\\    \kw{tracecase}~\texttt{Lit}~M~\kw{of}\ (x.M_L, M_I, M_F, M_C, M_E, M_P)
                     &\leadsto M_L[x \coloneqq M] \\
    \kw{tracecase}~\texttt{If}~M~\kw{of}\ (M_L, x.M_I, M_F, M_C, M_E, M_P)
                     &\leadsto M_I[x \coloneqq M] \\
    \kw{tracecase}~\texttt{For}~C~M~\kw{of}\ (x.M_L, x.M_I, \alpha.x.M_F, x.M_C, \alpha.x.M_E, x.M_P)
                     &\leadsto M_F[\alpha \coloneqq C, x \coloneqq M] \\
    \kw{tracecase}~\texttt{Cell}~M~\kw{of}\ (x.M_L, x.M_I, \alpha.x.M_F, x.M_C, \alpha.x.M_E, x.M_P)
                     &\leadsto M_C[x \coloneqq M] \\
    \kw{tracecase}~\texttt{OpEq}~C~M~\kw{of}\ (x.M_L, x.M_I, \alpha.x.M_F, x.M_C, \alpha.x.M_E, x.M_P)
                     &\leadsto M_E[\alpha \coloneqq C, x \coloneqq M] \\
    \kw{tracecase}~\texttt{OpPlus}~M~\kw{of}\ (x.M_L, x.M_I, \alpha.x.M_F, x.M_C, \alpha.x.M_E, x.M_P)
                                           &\leadsto M_P[x \coloneqq M]\\
    \kw{typecase}~\texttt{Bool}~\kw{of}\ (M_B, M_I, M_S, \beta.M_L, \rho.M_R, \gamma.M_T)
                     &\leadsto M_B  \\
    \kw{typecase}~\intty~\kw{of}\ (M_B, M_I, M_S, \beta.M_L, \rho.M_R, \gamma.M_T)
                     &\leadsto M_I  \\
    \kw{typecase}~\texttt{String}~\kw{of}\ (M_B, M_I, M_S, \beta.M_L, \rho.M_R, \gamma.M_T)
                     &\leadsto M_S  \\
    \kw{typecase}~\texttt{List}~C~\kw{of}\ (M_B, M_I, M_S, \beta.M_L, \rho.M_R, \gamma.M_T)
                     &\leadsto M_L[\beta \coloneqq C] \\
    \kw{typecase}~\texttt{Record}~S~\kw{of}\ (M_B, M_I, M_S, \beta.M_L, \rho.M_R, \gamma.M_T)
                     &\leadsto M_R[\rho \coloneqq S] \\
    \kw{typecase}~\texttt{Trace}~C~\kw{of}\ (M_B, M_I, M_S, \beta.M_L, \rho.M_R, \gamma.M_T)
                     &\leadsto M_T[\gamma \coloneqq C] \\
  \end{align*}

  \caption{Normalization $\beta$-rules. See also commuting conversions in Figure~\ref{fig:normalization-cc}, congruence rules in Figure \ref{fig:normalization-rules-congruence}, and constructor computation rules in Figure~\ref{fig:constructor-computation} }
  \label{fig:normalization-beta}
\end{figure*}

\begin{figure*}
  \footnotesize
  \begin{align*}
    (\kw{if}~L~\kw{then}~M_1~\kw{else}~M_2)\ N &\leadsto \kw{if}~L~\kw{then}~M_1\ N~\kw{else}~M_2\ N \\
    (\kw{if}~L~\kw{then}~M_1~\kw{else}~M_2)\ C &\leadsto \kw{if}~L~\kw{then}~M_1\ C~\kw{else}~M_2\ C \\
    (\kw{if}~L~\kw{then}~M~\kw{else}~N).l &\leadsto \kw{if}~L~\kw{then}~M.l~\kw{else}~N.l \\
    \kw{for}~(x \leftarrow M_1 \concat M_2)~N &\leadsto (\kw{for}~(x \leftarrow M_1)~N) \concat (\kw{for}~(x \leftarrow M_2)~N) \\
    \kw{for}~(x \leftarrow \kw{for}~(y \leftarrow L)~M)~N &\leadsto \kw{for}~(y \leftarrow L)~\kw{for}~(x \leftarrow M)~N
\\
                \kw{if}~(\kw{if}~L~\kw{then}~M_1~\kw{else}~M_2)~\kw{then}~N_1~\kw{else}~N_2 
                &\leadsto \kw{if}~L~\kw{then}~(\kw{if}~M_1~\kw{then}~N_1~\kw{else}~N_2)~\kw{else}~(\kw{if}~M_2~\kw{then}~N_1~\kw{else}~N_2) \\[.5\baselineskip]
                \kw{for}~(x \leftarrow \kw{if}~L~\kw{then}~M_1~\kw{else}~M_2)~N 
                & \leadsto \kw{if}~L~\kw{then}~\kw{for}~(x \leftarrow M_1)~N~\kw{else}~\kw{for}~(x \leftarrow M_2)~N \\[.5\baselineskip]
                \kw{tracecase}~\kw{if}~L~\kw{then}~M_1~\kw{else}~M_2~\kw{of}\ (M_L, M_I, M_F, M_C, M_E, M_P) 
                & \leadsto \kw{if}~L~\kw{then}~\kw{tracecase}~M_1~\kw{of}\ (M_L, M_I, M_F, M_C, M_E, M_P)\\
                & \qquad \quad \kw{else}~\kw{tracecase}~M_2~\kw{of}\ (M_L, M_I, M_F, M_C, M_E, M_P)
  \end{align*}

  \caption{Commuting conversions reorder expressions to expose more $\beta$-reductions.}% See also $\beta$-rules in Figure~\ref{fig:normalization-beta}, constructor computation rules in Figure~\ref{fig:constructor-computation}, and congruence rules in Figure \ref{fig:normalization-rules-congruence}.}
  \label{fig:normalization-cc}
\end{figure*}

Reduction rules fall into one of three categories:
$\beta$-rules are listed in Figure~\ref{fig:normalization-beta} and perform computation when introduction and elimination forms meet, like application of a function, or projection out of a record;
commuting conversions, listed in Figure~\ref{fig:normalization-cc}, reorder terms to expose more $\beta$-reductions;
and congruence rules (Figure~\ref{fig:normalization-rules-congruence}) allow subterms to reduce independently.
For example, \lstinline|(if x then {a = 5} else y).a| reduces by a commuting conversion to \lstinline|if x then {a = 5}.a else y.a|.
A $\beta$-rule reduces \lstinline|{a = 5}.a| to \lstinline|5| and a congruence rule allows this reduction to happen inside the \lstinline|then| branch.
Thus the whole term reduces to \lstinline|if x then 5 else y.a|.

Unlike in standard evaluation rules, we perform reduction under binders, like functions and comprehensions and, as seen above, in the branches of if-then-else.
This is crucial for removing all occurrences of language constructs that we cannot translate to \SQL because comprehension bodies and conditionals can of course remain in the result of normalization.

The reduction rules do not impose any particular order of execution, like call-by-name or call-by-value, but since all operations are pure, this is not observable.

\subsection{Preservation}\label{sec:tlinks-preservation}

To prove preservation we will need the following substitution lemmas.
Substitution of variables in terms (1), type variables in types (2), and type variables in terms (4) are standard for \lamiml \citep{morrisett1995compiling,crary_weirich_morrisett_2002}.
We add variants for row constructors: substitution of row variables in types (3), a variant of (2); and substitution of row variables in terms (5), a variant of (4).
The row variants use the syntactic sort $S$ in place of $C$ and $\rho$ instead of $\alpha$.

\begin{lemma}[Substitution lemmas]\label{lem:substitution-lemmas}
  ~
  \begin{enumerate}
  \item If $\Gamma, x:A \vdash M: B$ and $\Gamma \vdash N:A$ then $\Gamma \vdash M[x\coloneqq N]:B$.
  \item If $\Gamma, \alpha:K \vdash A: K'$ and $\Gamma \vdash C:K$ then $\Gamma[\alpha \coloneqq C] \vdash A[\alpha \coloneqq C]:K'[\alpha \coloneqq C]$.
  \item If $\Gamma, \rho:K \vdash A: K'$ and $\Gamma \vdash S:K$ then $\Gamma[\rho \coloneqq S] \vdash A[\rho \coloneqq S]:K'[\rho \coloneqq S]$.
  \item If $\Gamma, \alpha:K \vdash M: A$ and $\Gamma \vdash C:K$ then $\Gamma[\alpha \coloneqq C] \vdash M[\alpha \coloneqq C]:A[\alpha \coloneqq C]$.
  \item If $\Gamma, \rho:K \vdash M: A$ and $\Gamma \vdash S:K$ then $\Gamma[\rho \coloneqq S] \vdash M[\rho \coloneqq S]:A[\rho \coloneqq S]$.
  \end{enumerate}
\end{lemma}

We also need standard context manipulation lemmas for weakening and swapping the order of unrelated variables.

\begin{lemma}[Weakening]\label{lem:weakening}
  If $\Gamma \vdash M : A$, $\Gamma \vdash B : K$, and $x$ does not appear free in $\Gamma$, $M$, $A$, then $\Gamma, x:B \vdash M:A$.
\end{lemma}

\begin{lemma}[Context swap]\label{lem:context-swap}
  If $\Gamma, x:A_x, y:A_y \vdash M : B$ and $x$ does not appear free in $A_y$ then $\Gamma, y:A_y, x:A_x \vdash M : B$.
\end{lemma}

With these helper lemmas out of the way, we can prove that the reduction relation $\leadsto$ preserves kinds of constructors and types of terms.

\begin{lemma}[Constructor preservation]\label{lem:preservation-constructor}
  For all \TLinks type constructors $C$ and row constructors $S$, contexts $\Gamma$, and kinds $K$, if $\Gamma \vdash C : K$ and $C \leadsto C'$, then $\Gamma \vdash C' : K$ and if $\Gamma \vdash S : K$ and $S \leadsto S'$, then $\Gamma \vdash S' : K$.
\end{lemma}

\begin{lemma}[Preservation]\label{lem:preservation}
  For all \TLinks terms $M$ and $M'$, contexts $\Gamma$, and types $A$, if $\Gamma \vdash M : A$ and $M \leadsto M'$, then $\Gamma \vdash M' : A$.
\end{lemma}

\subsection{\TLinks normal form}\label{sec:tlinks-normal-form}

\begin{figure}
  \footnotesize
  \[
    \begin{array}{lrcl}
      \text{Normal constructors} & C & \Coloneqq & E \mid \texttt{Bool}^* \mid \inttyc \mid \texttt{String}^* \mid \lambda \alpha: K.C \\
                          & & \mid & \texttt{List}^*\ C \mid \texttt{Record}^*\ S \mid \texttt{Trace}^*\ C \\
      \text{Neutral constructors} & E & \Coloneqq & \alpha \mid E\ C \mid \kw{Typerec}~E~ (C_B, C_I, C_S, C_L, C_R, C_T) \\
      \text{Normal row constr.}  & S & \Coloneqq & \cdot \mid l : C; S \mid U \\
      \text{Neutral row constr.} & U & \Coloneqq & \rho \mid l : C; U \mid \kw{Rmap}\ C\ U \\

      \text{Normal terms} & M, N & \Coloneqq & F \mid c \mid \lambda x:A.M \mid \Lambda \alpha:K.M \\
                          & & \mid & \kw{if}~H~\kw{then}~M~\kw{else}~N \mid M + N \\
                          & & \mid & \langle \rangle \mid \langle l = M; N \rangle \mid \kw{rmap}^U~M~N \\
                          & & \mid & [] \mid [M] \mid M \concat N \mid \kw{for}~(x \leftarrow T)~N \mid \kw{table}~n~\langle R \rangle \\
                          & & \mid & \texttt{Lit}\ M \mid \texttt{If}\ M \mid \texttt{For}\ C\ M \mid \texttt{Cell}\ M \mid \texttt{OpEq}\ C\ M \mid \texttt{OpPlus}\ M \\
      \text{Neutral terms} & F & \Coloneqq & x \mid P.l \mid F\ M \mid F\ C \mid \kw{rfold}^U~L~M~N \\
                          & & \mid & \kw{tracecase}~F~\kw{of}~(x.M_L, x.M_I, \alpha.x.M_F, x.M_C, \alpha.x.M_E, x.M_P) \\
                          & & \mid & \kw{typecase}~E~\kw{of}~(M_B, M_I, M_S, \beta.M_L, \rho.M_R, \beta.M_T) \\
      \text{Neutral conditional} & H & \Coloneqq & F \mid M == N \\
      \text{Neutral projection} & P & \Coloneqq & F \mid \kw{rmap}^U~M~N \\
      \text{Neutral table} & T & \Coloneqq & F \mid \kw{table}~n~\langle R \rangle
    \end{array}
  \]
  \caption{\TLinks normal form.}
  \label{fig:tlinks-normal-form}
\end{figure}

Unlike in typical progress and preservation proofs, our goal is not to reduce a program to a value like a number, string, or even a closure.
Rather, we perform rewriting to partially evaluate parts of the program that are independent of values in the database.
The goal is in particular to eliminate all occurrences of language constructs we cannot translate to \SQL.
The \TLinks normal form is a crucial component of the argument for success.
In combination with the progress lemma in the next section, it tells us what terms look like after exhaustive application of the normalization rules.
Compared to \TLinks source terms, the \TLinks normal form shows that certain combinations of expressions are impossible after normalization, like an application of a literal function.
Other terms necessarily remain, like iteration over a table (but not a literal list).
We also see that some constructs are in normal form that are not in our target, the nested relational calculus.
We will later argue that these cannot actually appear in queries, usually because queries are closed and have restricted types.

The grammar of \TLinks normal forms is given in Figure \ref{fig:tlinks-normal-form}.
Constructors $C$ in \TLinks normal form differ from constructors in non-normal \TLinks in the application and \lstinline|Typerec| forms.
The idea is that the normal form only includes type applications and \lstinline|Typerec| forms which are blocked from further reduction by an unbound type variable.
For example, $(\lambda \alpha.\mathtt{Bool}^*)\ \mathtt{Int}^*$ is not in \TLinks normal form (and we do not want it to be in normal form, because it can reduce to $\mathtt{Bool}^*$).
On the other hand, $\alpha\ \mathtt{Int}^*$ is stuck and in normal form.

\begin{remark}\label{remark:constructors-free-type-variable}
  Constructors $E$ and row constructors $U$ always contain at least one free type variable $\alpha$ or $\rho$ and those are the only base cases for their respective sort.
\end{remark}
We will later use the above to show that some term forms are impossible within closed query terms in normal form.
Such terms do not contain free type variables, so $E$ and $U$ collapse into nothing, and terms built from $E$ and $U$ (like \lstinline|rmap|) cannot appear.

Neutral terms $F$ are those stuck on a free variable $x$, a stuck constructor $E$, or a stuck row constructor $U$.
We also restrict what can appear as the condition in an if-then-else, the iteratee of a list comprehension, and in the record position of a projection.
We will later argue that in a query term, all variables are references into tables and therefore everything that is not nested relational calculus will disappear.
The reason for having separate syntactic sorts $H$, $P$, and $T$ is to make this argument independent of types.

\subsection{Progress}\label{sec:tlinks-progress}

In this section we prove progress lemmas:
a well-typed \TLinks term is either in normal form or it reduces to some other term, and similarly for constructors and row constructors.
The proofs are not surprising --- all of the creative work is in the reduction relations and normal forms.

% \james{Might be worth pointing out the similarities and differences with "standard" progress/preservation:
% - reduction under lambda, inside comprehensions etc.
% - goal is not just to ensure lack of "stuckness" but that the normal forms are suitable input for later query compilation stages
% - we might also want to prove termination/strong normalization (subject to some caveat about recursion) but that would be a lot of effort for relatively little practical benefit.}

\begin{lemma}[Constructor and row constructor progress]\label{lem:progress-constructor}
  For all well-kinded \TLinks type constructors $C$ and row constructors $S$, we have that they are either in \TLinks normal form (Figure \ref{fig:tlinks-normal-form}), or there is a type constructor $C'$ with $C \leadsto C'$, or row constructor $S'$ with $S \leadsto S'$, respectively.
\end{lemma}

\begin{lemma}[Progress]\label{lem:progress}
  For all well-typed \TLinks terms $M$, either $M$ is in \TLinks normal form (Figure \ref{fig:tlinks-normal-form}), or there is a \TLinks term $M'$ with $M \leadsto M'$.
\end{lemma}

\subsection{Queries normalize to nested relational calculus}\label{sec:tlinks-tighten}

In this section, we further restrict the \TLinks normal form for queries, that is, closed expressions of nested relational type.
The general idea is, that because queries are closed and have nested relational type, they cannot possibly contain functions, polymorphism, record map, etc.
The proof relies heavily on the exact definition of the normal form.
In particular, the sorts $U$ and $E$ (Figure \ref{fig:tlinks-normal-form}) have type and row variables as the only base cases.
Queries in normal form do not contain any type or row variables and therefore do not contain any terms that are built using $U$ or $E$, like \lstinline|rmap| or \lstinline|typecase|.
We cannot rid ourselves of term variables --- and thus terms they appear in --- in quite the same manner, because \lstinline|for|-comprehensions bind term variables and can appear in normal forms (and indeed must appear, otherwise we would have no need for generating database queries in the first place).
However, since queries are closed, the only variables that appear are bound by comprehensions over tables and thus have closed record types with labels of base types.
We capture this property in the definition of query contexts (Definition~\ref{def:query-context}).
We can use this to show a lemma which states that all neutral terms $F$ are actually variables or projections of variables.
We use this lemma to argue that queries are free of, for example, applications $F\ M$, because $F$ collapses to $x$ or $x.l$ and we know that all variables have table row types (closed records with labels of base type) and thus the application would be ill-typed.
This argumentation extends to the other constructs that are in \TLinks normal form but not in nested relational calculus, and therefore we conclude that closed queries in normal form are in nested relational calculus.

\begin{definition}[Query context]\label{def:query-context}
  A query context does not contain type or row variables and all term variables have closed record type with labels of base type.

  \begin{itemize}
  \item The empty context $\cdot$ is a query context.
  \item The context $\Gamma, x:\langle \overline{l_i : A_i} \rangle$ is a query context, if $\Gamma$ is a query context, $x$ is not bound in $\Gamma$ already, and each type $A_i$ is a base type.
  \end{itemize}
\end{definition}

\begin{lemma}\label{lem:f-collapses}
  A term in normal form $F$ (Figure \ref{fig:tlinks-normal-form}) that matches the grammar for $F$ and is well-typed in a query context $\Gamma$, is of the form $x$ or $x.l$.
\end{lemma}

\begin{figure}
  \footnotesize
  \[
    \begin{array}{lrcl}
      \text{Types} & A & \Coloneqq & \mathtt{Bool} \mid \mathtt{Int} \mid \mathtt{String} \mid [A] \mid \langle\overline{l:A}\rangle \\
      \text{Terms} & M, N, L & \Coloneqq & c \mid x \mid \langle \overline{l = M} \rangle \mid M.l \mid M + N \mid M == N \mid \kw{if}~L~\kw{then}~M~\kw{else}~N \\
                   & & \mid & [] \mid [M] \mid M \concat N \mid \kw{for}~(x \leftarrow N)~M \mid \kw{table}\ n\ \langle \overline{l: A} \rangle
    \end{array}
  \]
  \caption{Target normal form for queries: \NRC.}
  \label{fig:normalization-target-normal-form}
\end{figure}

\begin{theorem}\label{thm:nf-query-nrc}
  If $M$ is a term in \TLinks normal form with a nested relational type in a query context $\Gamma$, then $M$ is in the nested relational calculus (Figure \ref{fig:normalization-target-normal-form}).
\end{theorem}

% Obviously recursive functions are not strongly normalizing in general.

% There is nothing we can do about that.
% One common solution is to enforce structural recursion syntactically, like \Coq, \Idris, and others do.
% The other solution is to use the bound on the depth of a traced query to unroll fixpoints.
% One important aspect of this is that there is no pattern matching on lists, so the bound on the depth is actually enough, even though values are possibly \emph{large}, i.e. database-sized, not query-sized, but the same is true in plain \Links.
% \stefan{Actually, the \Links issue tracker says that pattern matching on lists always typechecks as databasable, but compiles to \lstinline|hd| and \lstinline|tl| and does not actually work. I wonder why.}

% I think a translation to \Idris is reasonably straightforward, but \Idris does not normalize under binders and does not have commuting conversions to deal with \kw{for}-comprehensions blocking reduction.
% Given a normalization proof, adding commuting conversions \emph{should} be easy for someone who knows what they are doing.
% \stefan{Unfortunately, I don't, and that's the only real issue here.}

% \Idris is a very high-level language to translate to.
% We do not need to encode for example the list type as a sum of unit and the type argument or any such tedious nonsense.
% In a way that is a good thing.
% It also answers James McKinna's question: ``Would dependent types help?''
% Or, what would all of this look like if you \emph{had} dependent types?

\section{Implementation}\label{sec:tlinks-implementation}

We implemented a prototype of the \TLinks self-tracing transformation and normalization procedure in \Haskell.
We also implemented the \lstinline|value|, \lstinline|wherep|, and \lstinline|lineage| trace analysis functions, as described in Section~\ref{sec:trace-analyses}.
This is just enough to report some initial results on provenance through trace analysis on a couple of examples.

Recall the boat tours query from Figure~\ref{fig:boat-tours}.
The query below is a minor variant (with reordered comprehensions and moved conditions) in \TLinks.
\begin{lstlisting}
for (x <- table "agencies" {..})
for (y <- table "externalTours" {..})
  if (x.name == y.name && y.type == "boat")
  then [{name = y.name, phone = x.phone}] else []
\end{lstlisting}
We can report that tracing the above query, applying the \lstinline|value| trace analysis function, and normalizing again results in the exact same query.

More interestingly, we can trace the query and apply the \lstinline|wherep| trace analysis function to extract where-provenance.
The normalized query is shown below.
The representation of where-provenance in \TLinks's \lstinline|wherep| is slightly different from \WLinks, but the queries are very close.
\begin{lstlisting}
for (x <- table "agencies" {..})
for (y <- table "externalTours" {..})
  if (x.name == y.name && y.type == "boat")
  then [{name = {%table% = "externalTours", column = "name",
                 row = y.oid, data = y.name},
         phone = {%table% = "agencies", column = "phone",
                  row = x.oid, data = x.phone}}]
  else []
\end{lstlisting}

Doing the same with \lstinline|lineage| once again shows the problem with tracing at the leaves and combining annotations using concatenation:
Every row of the boat tours example has 15 lineage annotations, instead of 2, as seen below.
\begin{lstlisting}
for (x <- table "agencies" {..})
for (y <- table "externalTours" {..})
  if (x.name == y.name && y.type == "boat")
  then [{data = {name = y.name, phone = x.phone},
         lineage = [{%table% = "agencies", row = x.oid}] ++
                   [{%table% = "agencies", row = x.oid}] ++
                   [{%table% = "agencies", row = x.oid}] ++
                   [{%table% = "externalTours", row = y.oid}] ++
                   [{%table% = "externalTours", row = y.oid}] ++
                   [{%table% = "externalTours", row = y.oid}] ++
                   [{%table% = "externalTours", row = y.oid}] ++
                   [{%table% = "externalTours", row = y.oid}] ++
                   [{%table% = "agencies", row = x.oid}] ++
                   [{%table% = "agencies", row = x.oid}] ++
                   [{%table% = "agencies", row = x.oid}] ++
                   [{%table% = "externalTours", row = y.oid}] ++
                   [{%table% = "externalTours", row = y.oid}] ++
                   [{%table% = "externalTours", row = y.oid}] ++
                   [{%table% = "externalTours", row = y.oid}] ++
                   [{%table% = "agencies", row = x.oid}]}]
  else []
\end{lstlisting}

We did not implement set semantics, or a special operator to remove static duplication.
Something along those lines is clearly needed for provenance based on trace analysis.

Below is a variant of the example query from Chapter~\ref{cha:llinks}, after being traced, analyzed with the \lstinline|value| trace analysis function, and normalized.
Again, normalization removes all traces of tracing and results in a reasonable query.
\begin{lstlisting}
for (x <- table "presidents" {nth: Int, name: String})
  [{dates = for (y <- table "inaugurations" {..})
            for (z <- table "metro" {..})
              if (y.nth == x.nth && z.date == y.date &&
                  z.time == 11 && z.trips >= 193000)
              then [y.date] else [],
    name = x.name}]
\end{lstlisting}

where-provenance of nested results works, as seen below.
\begin{lstlisting}
for (x <- table "presidents" {nth: Int, name: String})
  [{dates = for (y <- table "inaugurations" {..})
            for (z <- table "metro" {..})
              if (y.nth == x.nth && z.date == y.date &&
                  z.time == 11 && z.trips >= 193000)
              then [{%table% = "inaugurations", column = "date",
                     row = y.oid, data = y.date}]
              else [],
    name = {%table% = "presidents", column = "name",
            row = x.oid, data = x.name}}]
\end{lstlisting}

Figure~\ref{fig:q-lineage} shows the normalized query after tracing and applying the \lstinline|lineage| trace analysis function.
This time, we removed the obviously duplicated lineage annotations.
Still, the last line adds the presidents table to the lineage of the outer collection.
This is one instance where static deduplication in set union is not entirely trivial.
We would have to push the singleton list with the presidents annotation into the nested comprehensions and into the else-branch (the then-branch stays as it is) to entirely remove duplicates.

\begin{figure}
\begin{lstlisting}
for (x <- table "presidents" {nth: Int, name: String})
  [{data = {dates = for (y <- table "inaugurations" {..})
                    for (z <- table "metro" {..})
                      if (y.nth == x.nth && z.date == y.date &&
                          z.time == 11 && z.trips >= 193000)
                      then [{data = y.date,
                             lineage = [{%table% = "presidents",
                                         row = x.oid},
                                        {%table% = "inaugurations",
                                         row = y.oid},
                                        {%table% = "metro",
                                         row = z.oid}]}]
                      else [],
            name = x.name},
    lineage = (for (y <- table "inaugurations" {..})
               for (z <- table "metro" {..})
                 if (y.nth == x.nth && z.date == y.date &&
                     z.time == 11 && z.trips >= 193000)
                 then [{%table% = "presidents", row = x.oid},
                       {%table% = "inaugurations", row = y.oid},
                       {%table% = "metro", row = z.oid}]
                 else []) ++
              [{%table% = "presidents", row = x.oid}]}]
\end{lstlisting}
  \caption{Trace analysis with \texttt{lineage} of the example query from Chapter~\ref{cha:llinks} with obvious lineage annotation duplication manually removed.}
  \label{fig:q-lineage}
\end{figure}

We also tried some of the benchmark queries from Chapter~\ref{cha:evaluation}.
Other than the duplication of annotations in the lineage queries, the generated code looks reasonable.
Normalization performance is good enough to be unnoticeable, even with a naive implementation of the reduction rules that only performs a single step at a time and re-traverses the expression until it finds the next redex in every step.

\section{Related and future work}\label{sec:tlinks-related-future}

We did not prove strong normalization and in the presence of \lstinline|fix| we do not expect strong normalization to hold.
However, it would be nice to have some guarantee about the termination behavior of normalization like: if call-by-name evaluation would terminate then normalization terminates.
Then, an implementation could use this to guarantee termination of trace analysis functions by, for example, enforcing structural recursion.

Extracting provenance from traces is not a new idea \citep{10.1007/978-3-642-28641-4_22,cheney14ppdp,misinterpretingsql}.
What makes our work different is that traces and trace analysis are defined in the language itself.
In combination with query normalization, this makes \TLinks the first, to our knowledge, system that can execute user-defined query trace analysis on the database.

Compared to some of the other work on tracing, our traces contain less information.
Some information would be easy to add, like concatenation operations or projections.
Other information requires changing the structure of traces in a more invasive way.
In particular, our traces are cell-level only and do not include information about the binding structure of queries.
We also trace only after a first normalization phase, so traces do not include information about, for example, functions in the original query code.
Tree-shaped traces with explicit representation of variables like those proposed by \citet{cheney14ppdp} in particular, seem to make writing well-typed provenance extraction functions more difficult.
It can be done with dependent types --- we prototyped such traces and trace analysis functions in \Idris --- but this is not necessarily the direction we expect \Links to go.
\citet{misinterpretingsql} only record dynamic control flow decisions in traces and interpret the static query together with the dynamic trace to recover provenance.
It would be interesting to see whether we could do something similar in a more language-integrated way.

We propose to use query shredding \citep{SIGMOD2014CheneyLW} to turn nested relational calculus into a bounded number of \SQL queries because it is implemented in \Links already.
Alternatively, we could use other query compilation strategies like that employed by \DSH \citep{SIGMOD2015UlrichG} which is based on the flattening transformation \citep{JPDC1990BlellochS} or even target other execution backends by translating nested relational calculus further using, for example, the query compiler \QCert \citep{Auerbach:2017:PQC:3136534.3110253}.

\TLinks follows \Links tradition and uses a normalization procedure that eliminates language constructs with no obvious counterpart in \SQL, rather than attempt to encode these constructs.
However, the latter might be an option too.
\citet{crary_weirich_morrisett_2002} introduce $\lambda_r$, a variant of \lamiml where runtime type information is explicitly represented as a datatype when necessary.
\citet{DDFP2013GiorgidzeGUW} show how to translate algebraic datatypes to \SQL and \citet{DBPL2013GrustU} translate functions to \SQL.
It seems plausible that one could put these together to translate all of \TLinks to \SQL without necessarily normalizing to eliminate functions, traces, and typecase.
Indeed, the restriction to query types would become unnecessary.
One might still want to do some normalization, or partial evaluation, to avoid computing large traces where possible.

\TLinks builds on \lamiml \citep{morrisett1995compiling}.
\lamr improves on \lamiml in making runtime type information explicit, avoiding passing types where unnecessary, and improving the ergonomics of the typecase typing rule by refining types in context \citet{crary_weirich_morrisett_2002}.
An implementation would benefit from the latter.
The former points do not matter much in the context of \Links, because it is interpreted anyway, which makes it easy to access to type information at runtime, and we expect normalization time to typically be irrelevant compared to the time it takes to open a database connection, let alone execute a query.

\TLinks features generic record programming in the form of record mapping and folding.
These were the simplest extensions to how \Links currently implements records and row types \citep{TLDI2012LindleyC} we could come up with, that would meet the requirements of trace analysis.
Other languages with generic record programming constructs include \Urweb and \Purescript.

\Urweb \citep{POPL2015Chlipala} features ``first class, type-level names and records'' \citep{PLDI2010Chlipala}.
Its generic and metaprogramming features seem suitable for our needs but again, dependent types are a drastic extension to \Links's current type system.
Type inference for \TLinks is an open problem.
Type inference for \Urweb is undecidable.
However, \citet{PLDI2010Chlipala} claims that heuristics work well-enough in practice to mostly avoid proof terms and complex type annotations.
Maybe this could be a model for \TLinks, too.

\Purescript is a \Haskell-like language with first class records based on row types.
It supports generic record programming by converting back and forth between rows and type-level lists, and general type-level computation with multi-parameter type classes, functional dependencies, and parts of instance chains \citep{Morris:2010:ICT:1863543.1863596}.
This is enough to encode type-level functions like \lstinline|WHERE|, but not a particularly direct or pleasant way to program.
\Links does not at the moment have anything like type classes.
It is not clear that implementing all of this machinery just to avoid record map and fold is cost-effective.
However, type classes are widely useful in general and we could also use them to restrict queries to query types instead of having this built into the typechecker, so it might be worthwhile.

\Haskell does not have any particular record support worth mentioning.
Even so, it is almost certainly possible to encode these things in \Haskell and it would be interesting to see an implementation of \TLinks on top of \DSH \citep{IFL2010GiorgidzeGSW,SIGMOD2015UlrichG,Programming2018StolarekC}.

As mentioned before, we have designed \TLinks to be as easy an extension of \Links as possible, but it is not implemented yet.
This should probably be the next step towards flexible, efficient, and effective language-integrated provenance.

\section{Appendix}

\subsection{Proof of Lemma~\ref{lem:valuetf-inverse}}
\begin{proof}
  By induction on query types $C$ and closed rows of query types $S$.
  \begin{itemize}
  \item Base types \texttt{Bool}$^*$, \intty$^*$, \texttt{String}$^*$:
    \[ \mathtt{VALUE}(\mathtt{TRACE}\ \mathtt{Bool}^* )
      = \mathtt{VALUE}(\mathtt{Trace}\ \mathtt{Bool}^* )
      = \mathtt{Bool}^*
    \]
  \item List types \texttt{List}$^*$ $D$:
    \begin{align*}
      \mathtt{VALUE}(\mathtt{TRACE}\ (\mathtt{List}^*\ D))
      &= \mathtt{VALUE}(\mathtt{List}^*\ (\mathtt{TRACE}\ D)) \\
      &= \mathtt{List}^*\ (\mathtt{VALUE}(\mathtt{TRACE}\ D)) \\
      &= \mathtt{List}^*\ D
    \end{align*}
  \item Record types \texttt{Record}$^*\ S$:
    \begin{align*}
      \mathtt{VALUE}(\mathtt{TRACE}\ (\mathtt{Record}^*\ S))
      &= \mathtt{VALUE}(\mathtt{Record}^* (\kw{Rmap}\ \mathtt{TRACE}\ S)) \\
      &= \mathtt{Record}^*\ (\kw{Rmap}\ \mathtt{VALUE}\ (\kw{Rmap}\ \mathtt{TRACE}\ S)) \\
      &= \mathtt{Record}^*\ S
    \end{align*}
  \item Empty row $\cdot$: $\kw{Rmap}\ \mathtt{VALUE}\ (\kw{Rmap}\ \mathtt{TRACE}\ \cdot) = \cdot$
  \item Row cons $(l:A, S)$:
    \begin{align*}
      & \kw{Rmap}\ \mathtt{VALUE}\ (\kw{Rmap}\ \mathtt{TRACE}\ (l:A, S)) \\
      =& \kw{Rmap}\ \mathtt{VALUE}\ (l:\mathtt{TRACE}\ A, \kw{Rmap}\ \mathtt{TRACE}\ S) \\
      =& (l:\mathtt{VALUE}\ (\mathtt{TRACE}\ A), \kw{Rmap}\ \mathtt{VALUE}\ (\kw{Rmap}\ \mathtt{TRACE}\ S)) \\
      =& (l:A, \kw{Rmap}\ \mathtt{VALUE}\ (\kw{Rmap}\ \mathtt{TRACE}\ S)) \\
      =& (l:A, S)
    \end{align*}\qedhere
  \end{itemize}
\end{proof}

\subsection{Proof of Lemma~\ref{lem:trace-non-base}}
\begin{proof}
  By induction on query types $C$ made up from base types, lists, and closed records.
  Applying \lstinline|TRACE| to base types \lstinline|Bool|, \lstinline|Int|, and \lstinline|String| results in traced base types \lstinline|Trace Bool|, \lstinline|Trace Int|, and \lstinline|Trace String|, respectively.
  List types are guarded by the \lstinline|List| type constructor, and similarly for records.
  Traces are not query types, but if they were, the induction hypothesis would apply.
\end{proof}

\subsection{Proof of Lemma~\ref{lem:dist-type-correctness}}

\begin{proof}
  By induction on the query type $C$.

  \begin{itemize}
  \item The base cases are $\texttt{Bool}$, $\intty$, and $\texttt{String}$.
    For any base type $O$ out of these, we have $\texttt{TRACE}\ O = \texttt{Trace}\ O$.
    We have \[\mathit{dist}(\texttt{Trace}\ O, k) = \lambda t:\texttt{Trace}\ O.k[\mathbb{H} \coloneqq t]\] and need to show that it has type $\texttt{Trace}\ O \rightarrow \texttt{Trace}\ O$.
    Applying the $\lambda$-rule requires showing that the body has type $\texttt{Trace}\ O$.
    We instantiate the second hypothesis with $D = O$ and therefore have $\Gamma, \mathbb{H}:\texttt{Trace}\ O \vdash k:\texttt{Trace}\ O$.
    Both $t$ and $\mathbb{H}$ have type $\texttt{Trace}\ O$, so substituting one for the other in $k$ does not change the type (Lemma \ref{lem:substitution-lemmas}).

  \item Case $C = \texttt{List}\ (\texttt{TRACE}\ C')$:
    We need the right-hand side \[\lambda l:\texttt{List}\ (\texttt{TRACE}\ C').\kw{for}\ (x \leftarrow l)\ [\mathit{dist}(\texttt{TRACE}\ C', k)\ x] \] to have type $\texttt{TRACE}\ (\texttt{List}\ C') \rightarrow \texttt{TRACE}\ (\texttt{List}\ C')$.
    We use the rules for function abstraction, comprehension, singleton list, and application.
    We now need to show that $\mathit{dist}(\texttt{TRACE}\ C', k)$ has type $\texttt{TRACE}\ C' \rightarrow \texttt{TRACE}\ C'$ which is true by induction hypothesis with the same $k$.

  \item Case $C = \langle \overline{l:\texttt{TRACE}\ C'} \rangle$:
    The right-hand side \[\lambda r:\langle \overline{l:\texttt{TRACE}\ C'} \rangle.\langle \overline{ l = \mathit{dist}(\texttt{TRACE}\ C',k)\ (r.l) }\rangle\] needs to have type $\langle \overline{l:\texttt{TRACE}\ C'} \rangle \rightarrow \langle \overline{l:\texttt{TRACE}\ C'} \rangle$.
    Thus by function abstraction, record construction, record projection, and application we need each of the expressions $\mathit{dist}(\texttt{TRACE}\ C',k)$ to have type $\texttt{TRACE}\ C' \rightarrow \texttt{TRACE}\ C'$ which they do by induction hypothesis.
    \qedhere
  \end{itemize}
\end{proof}

\subsection{Proof of Theorem~\ref{thm:trace-type-correctness-2}}
\begin{proof}
  By induction on the typing derivation for $M : \texttt{T}(C)$.
  Almost all cases require that some subterms have a type $\mathtt{T}(C')$ that is equal to some query type $A$.
  We can obtain this constructor $C'$ by Lemma~\ref{lem:nrc-types-constr}.

  \begin{itemize}
  \item Case $\infer { Γ(x) = A } { Γ ⊢ x : A }$:
    $
      \infer
      {\trace{\Gamma}(x) = \mathtt{T}(\mathtt{TRACE}\ C) \quad \text{(Definition \ref{def:trace-context})}}
      {\trace{\Gamma} \vdash x : \mathtt{T}(\mathtt{TRACE}\ C)}
    $

  \item Literals $c$ have base types \lstinline|Bool|, \lstinline|Int|, or \lstinline|String|.
    Their traces \lstinline|Lit| $c$ have types \lstinline|Trace Bool|, \lstinline|Trace Int|, or \lstinline|Trace String|, respectively.

  \item Case $ \infer
    { Γ ⊢ L : \texttt{Bool} \\
      Γ ⊢ M : A \\
      Γ ⊢ N : A }
    { Γ ⊢ \kw{if}~L~\kw{then}~M~\kw{else}~N : A }$:

    The right hand side of the self-tracing transform is another \kw{if-then-else} with condition $\texttt{value (Trace Bool)}\ \trace{L}$ and then-branch
    \[
      \mathit{dist}(\texttt{TRACE}\ C, \texttt{If}\ \langle \texttt{cond} = \trace{L}, \texttt{out} = \mathbb{H} \rangle)\ \trace{M}
    \] and similar else-branch.

    In the condition, we apply $\texttt{value}: \forall\alpha.\texttt{T}(\alpha) \rightarrow \texttt{T}(\texttt{VALUE}\ \alpha)$ to a subtrace of type \lstinline|TRACE Bool| by induction hypothesis.
    Therefore it has type \lstinline|VALUE (TRACE Bool)| which is equal to \lstinline|Bool| by Lemma~\ref{lem:valuetf-inverse}.

    For all base types $D$, $\texttt{If}\ \langle \texttt{cond} = \trace{L}, \texttt{out} = \mathbb{H} \rangle$ has type $\texttt{Trace}\ D$ assuming $\mathbb{H}:\texttt{Trace}\ D$.
    Therefore, by Lemma~\ref{lem:dist-type-correctness}, the whole term in function position has type $\texttt{TRACE}\ C \rightarrow \texttt{TRACE}\ C$.
    We have $\trace{M}: \mathtt{T}(\mathtt{TRACE}\ C)$ by IH.
    The else-branch is analogous and the whole expression has type $\mathtt{T}(\mathtt{TRACE}\ C)$.

  \item Case $ \infer { } { Γ ⊢ [] : \texttt{List}\ A } $:
    \[
      \infer*
      {\infer*
        {\infer*
          { \trace{Γ} ⊢ \mathtt{T}(\mathtt{TRACE}\ C) : \mathit{Type} \text{ using } A = \mathtt{T}(C) }
          {
            \trace{Γ} ⊢ [] : \texttt{List}\ \mathtt{T}(\mathtt{TRACE}\ C)
          }
        }
        {\trace{Γ} ⊢ [] : \mathtt{T}(\texttt{List}^*\ (\mathtt{TRACE}\ C))}
      }
      {\trace{Γ} ⊢ [] : \mathtt{T}(\mathtt{TRACE}\ (\texttt{List}^*\ C))}
    \]

  \item Case $ \infer { Γ ⊢ M : A } { Γ ⊢ [M] : \texttt{List}\ A } $:
    \[
      \infer*
      { \infer*
        { \infer*
          { \text{IH} }
          { \trace{Γ} ⊢ \trace{M} : \mathtt{T}(\mathtt{TRACE}\ C)}
        }
        {
          \trace{Γ} ⊢ [\trace{M}]: \texttt{List}\ \mathtt{T}(\mathtt{TRACE}\ C)
        }
      }
      {
        \trace{Γ} ⊢ [\trace{M}]: \mathtt{T}(\mathtt{TRACE}\ (\texttt{List}^*\ C))
      }
    \]

  \item Case $ \infer
    { Γ ⊢ M : \texttt{List}\ A \and Γ ⊢ N : \texttt{List}\ A }
    { Γ ⊢ M \concat N  : \texttt{List}\ A }$:

    \[
      \infer*
      {
        \infer*
        {
          \infer*
          {
            \infer*
            { \text{IH} }
            { \trace{Γ} ⊢ \trace{M} : \mathtt{T}(\mathtt{TRACE}\ (\texttt{List}^*\ C)) }
          }
          { \trace{Γ} ⊢ \trace{M} : \texttt{List}\ \mathtt{T}(\mathtt{TRACE}\ C) } \and \text{ analogous for $N$}
        }
        { \trace{Γ} ⊢ \trace{M} \concat \trace{N} : \texttt{List}\ \mathtt{T}(\mathtt{TRACE}\ C) }
      }
      { \trace{Γ} ⊢ \trace{M} \concat \trace{N} : \mathtt{T}(\mathtt{TRACE}\ (\texttt{List}^*\ C)) }
    \]

  \item Case $ \infer
    { Γ ⊢ M : \texttt{List}\ B \\ Γ,x:B ⊢ N : \texttt{List}\ A }
    { Γ ⊢ \kw{for}~(x \leftarrow M)~N : \texttt{List}\ A } $:

    \[\footnotesize
      \infer*
      {
        \infer*
        { \infer*
          { \infer*
            { \text{IH} }
            { \trace{Γ} ⊢ \trace{M} : \mathtt{T}(\mathtt{TRACE}\ (\texttt{List}^*\ D)) }
          }
          { \trace{Γ} ⊢ \trace{M} : \mathtt{List}\ \mathtt{T}(\mathtt{TRACE}\ D) }
          \and
          \infer* { \star } {\trace{Γ},x:\mathtt{T}(\mathtt{TRACE}\ D) ⊢ b : \mathtt{List}\ \mathtt{T}(\mathtt{TRACE}\ C)} }
        { \trace{Γ} ⊢ \kw{for}~(x \leftarrow \trace{M})\ b : \texttt{List}\ \mathtt{T}(\mathtt{TRACE}\ C) }
      }
      { \trace{Γ} ⊢ \kw{for}~(x \leftarrow \trace{M})\ b : \mathtt{T}(\mathtt{TRACE}\ (\texttt{List}^*\ C)) }
    \]
    where $b = \mathit{dist}(\texttt{TRACE}\ C, \texttt{For}\ D\ \langle \texttt{in} = x, \texttt{out} = \mathbb{H} \rangle)\ \trace{N}$ and
    $\star$:

    \[
      \infer*
      { \infer*
        { \dagger
          \and
          \infer*
          { \text{IH} }
          { \trace{Γ},x:\mathtt{T}(\mathtt{TRACE}\ D) ⊢ \trace{N} : \mathtt{T}(\mathtt{TRACE}\ (\mathtt{List}^*\ C)) }
        }
        { \trace{Γ},x:\mathtt{T}(\mathtt{TRACE}\ D) ⊢ b : \mathtt{T}(\mathtt{TRACE}\ (\mathtt{List}^*\ C)) }
      }
      { \trace{Γ},x:\mathtt{T}(\mathtt{TRACE}\ D) ⊢ b : \mathtt{List}\ \mathtt{T}(\mathtt{TRACE}\ C) }
    \]

    $\dagger$: We have $\mathit{dist}(\texttt{TRACE}\ C, \texttt{For}\ D\ \langle \texttt{in} = x, \texttt{out} = \mathbb{H} \rangle)$ of type \[ \mathtt{T}(\mathtt{TRACE}\ (\mathtt{List}^*\ C)) \rightarrow \mathtt{T}(\mathtt{TRACE}\ (\mathtt{List}^*\ C))
    \]
    in context $\trace{Γ},x:\mathtt{T}(\mathtt{TRACE}\ D)$
    by Lemma~\ref{lem:dist-type-correctness}, because the partially applied trace constructor \texttt{For} has type \texttt{Trace}\ A' for all holes $\mathbb{H}:\mathtt{Trace}\ A'$.

  \item The case for records is similar to that for list concatenation, in that we have multiple subtraces where the induction hypothesis applies, we just collect them into a record instead of another list concatenation.

  \item Case record projection: The projection was well-typed before tracing, so the record term $M$ contains label $l$ with some type $A$.
    By induction hypothesis and $A = \mathtt{T}(\mathtt{TRACE}\ C)$ the trace of $M$ contains label $l$ with type \lstinline|TRACE $C$|.
    \[
        \infer
        { \infer
          { \text{IH} }
          { \trace{Γ} ⊢ \trace{M} : \langle l^\bullet: \texttt{T(TRACE $C$)}, \dots \rangle } }
        { \trace{Γ} ⊢ \trace{M}.l : \texttt{T(TRACE $C$)} }
      \]

  \item Case \kw{table}: This is a slightly more complicated version of the base case for constants.
    We essentially map the \texttt{Cell} trace constructor over every table cell.
    Thus we go from a list of records of base types to a list of records of \texttt{Trace}d base types.

    {\small
      \[\infer
        { \infer
          { \trace{Γ} ⊢ \kw{table}~\dots \\
            \infer*
            { \infer
              { \trace{Γ}, y:\langle\overline{l :C}\rangle ⊢ y.l : C
              }
              { \star }
            }
            { \trace{Γ}, y:\langle\overline{l :C}\rangle ⊢ [\langle\overline{l = \mathit{cell}(n, l, y.\texttt{oid}, y.l)}\rangle ] : [\langle\overline{l : \texttt{Trace}~C}\rangle] }
          }
          { \trace{Γ} ⊢ \kw{for}\ (y \leftarrow \kw{table}~n~\langle \overline{l : C} \rangle)~[\langle\overline{l = \mathit{cell}(n, l, y.\texttt{oid}, y.l)}\rangle ] : [\langle\overline{l : \texttt{Trace}~C}\rangle] }
        }
        { \trace{Γ} ⊢ \kw{for}\ (y \leftarrow \kw{table}~n~\langle \overline{l : C} \rangle)~[\langle\overline{l = \mathit{cell}(n, l, y.\texttt{oid}, y.l)}\rangle ] : \texttt{T(TRACE [$\langle\overline{l :C}\rangle$])}
        }
      \]
    }

    There are a couple of steps missing at $\star$.
    The singleton list step is trivial.
    Then we have one precondition for each column in the table.
    Recall that \textit{cell} is essentially an abbreviation for \lstinline!Cell!, which records table name, column name, row number, and the actual cell data in a trace.
    We use the table name $n$ and the record label $l$ as string values for the table and column fields.
    We enforce in the typing rules that every table has the \lstinline|oid| column of type \intty.

  \item Case equality:
    {\small
      \[
        \infer
        { \infer
          { }
          { \trace{Γ} ⊢ C : \mathit{Type}} \\
          \infer
          { \text{IH} }
          { \trace{Γ} ⊢ \trace{M} : \texttt{T(TRACE $C$)}} \\
          \infer
          { \text{IH} }
          { \trace{Γ} ⊢ \trace{N} : \texttt{T(TRACE $C$)}} \\
        }
        { \trace{Γ} ⊢ \texttt{OpEq}\ C\ \langle \texttt{left} = \trace{M}, \texttt{right} = \trace{N} \rangle : \texttt{Trace Bool} }
      \]
    }

  \item Case plus, with liberal application of \lstinline!T(TRACE Int) = Trace Int!:
    \[
      \infer
      { \infer
        { \text{Induction hypothesis} }
        { \trace{Γ} ⊢ \trace{M} : \texttt{T(TRACE Int)} } \\
        \infer
        { \text{Induction hypothesis} }
        { \trace{Γ} ⊢ \trace{N} : \texttt{T(TRACE Int)} } \\
      }
      { \trace{Γ} ⊢ \texttt{OpPlus}\ \langle \texttt{left} = \trace{M}, \texttt{right} = \trace{N} \rangle : \texttt{T(TRACE Int)} }
    \]
    \qedhere
  \end{itemize}
\end{proof}

\subsection{Congruence rules}
\begin{figure*}
\footnotesize
\centering
  \begin{align*}
    M \leadsto M' &\Rightarrow& \lambda x.M &\leadsto \lambda x.M' \\
    M \leadsto M' &\Rightarrow& M\ N &\leadsto M'\ N \\
    N \leadsto N' &\Rightarrow& M\ N &\leadsto M\ N' \\
    M \leadsto M' &\Rightarrow& \Lambda \alpha.M &\leadsto \Lambda \alpha.M' \\
    M \leadsto M' &\Rightarrow& M\ C &\leadsto M'\ C \\
    C \leadsto C' &\Rightarrow& M\ C &\leadsto M\ C' \\
    L \leadsto L' &\Rightarrow& \kw{if}~L~\kw{then}~M~\kw{else}~N &\leadsto \kw{if}~L'~\kw{then}~M~\kw{else}~N \\
    M \leadsto M' &\Rightarrow& \kw{if}~L~\kw{then}~M~\kw{else}~N &\leadsto \kw{if}~L~\kw{then}~M'~\kw{else}~N \\
    N \leadsto N' &\Rightarrow& \kw{if}~L~\kw{then}~M~\kw{else}~N &\leadsto \kw{if}~L~\kw{then}~M~\kw{else}~N' \\
    M\leadsto  M' &\Rightarrow& \langle l = M; N \rangle &\leadsto \langle l = M'; N \rangle \\
    N \leadsto  N' &\Rightarrow& \langle l = M; N \rangle &\leadsto \langle l = M; N' \rangle \\
    M \leadsto M' &\Rightarrow& M.l &\leadsto M'.l \\
    S \leadsto S' &\Rightarrow& \kw{rmap}^S\ M\ N &\leadsto \kw{rmap}^{S'}\ M\ N \\
    M \leadsto M' &\Rightarrow& \kw{rmap}^S\ M\ N &\leadsto \kw{rmap}^S\ M'\ N \\
    N \leadsto N' &\Rightarrow& \kw{rmap}^S\ M\ N &\leadsto \kw{rmap}^S\ M\ N' \\
    S \leadsto S' &\Rightarrow& \kw{rfold}^S\ L\ M\ N & \leadsto \kw{rfold}^{S'}\ L\ M\ N \\
    L \leadsto L' &\Rightarrow& \kw{rfold}^S\ L\ M\ N & \leadsto \kw{rfold}^S\ L'\ M\ N \\
    M \leadsto M' &\Rightarrow& \kw{rfold}^S\ L\ M\ N & \leadsto \kw{rfold}^S\ L\ M'\ N \\
    N \leadsto N' &\Rightarrow& \kw{rfold}^S\ L\ M\ N & \leadsto \kw{rfold}^S\ L\ M\ N' \\
    M \leadsto M' &\Rightarrow& [M] &\leadsto [M'] \\
    M \leadsto M' &\Rightarrow& M \concat N &\leadsto M' \concat N \\
    N \leadsto N' &\Rightarrow& M \concat N &\leadsto M \concat N' \\
    M \leadsto M' &\Rightarrow& M == N &\leadsto M' == N \\
    N \leadsto N' &\Rightarrow& M == N &\leadsto M == N' \\
    M \leadsto M' &\Rightarrow& M + N &\leadsto M' + N \\
    N \leadsto N' &\Rightarrow& M + N &\leadsto M + N' \\
    M \leadsto M' &\Rightarrow& \kw{for}~(x \leftarrow M)~N &\leadsto \kw{for}~(x \leftarrow M')~N \\
    N \leadsto N' &\Rightarrow& \kw{for}~(x \leftarrow M)~N &\leadsto \kw{for}~(x \leftarrow M)~N' \\
    M \leadsto M' &\Rightarrow& \texttt{Lit}\ M & \leadsto \texttt{Lit}\ M' \\
    M \leadsto M' &\Rightarrow& \texttt{If}\ M & \leadsto \texttt{If}\ M' \\
    C \leadsto C' &\Rightarrow& \texttt{For}\ C\ M & \leadsto \texttt{For}\ C'\ M \\
    M \leadsto M' &\Rightarrow& \texttt{For}\ C\ M & \leadsto \texttt{For}\ C\ M' \\
    M \leadsto M' &\Rightarrow& \texttt{Cell}\ M & \leadsto \texttt{Cell}\ M' \\
    C \leadsto C' &\Rightarrow& \texttt{OpEq}\ C\ M & \leadsto \texttt{OpEq}\ C'\ M \\
    M \leadsto M' &\Rightarrow& \texttt{OpEq}\ C\ M & \leadsto \texttt{OpEq}\ C\ M' \\
    M \leadsto M' &\Rightarrow& \texttt{OpPlus}\ M & \leadsto \texttt{OpPlus}\ M' \\
    M \leadsto M' &\Rightarrow& \kw{tracecase}~M~\kw{of}\ (M_L, M_I, M_F, M_C, M_E, M_P)
                     &\leadsto \kw{tracecase}~M'~\kw{of}\ (M_L, M_I, M_F, M_C, M_E, M_P) \\
    M_L \leadsto M_L' &\Rightarrow& \kw{tracecase}~M~\kw{of}\ (M_L, M_I, M_F, M_C, M_E, M_P)
                     &\leadsto \kw{tracecase}~M~\kw{of}\ (M_L', M_I, M_F, M_C, M_E, M_P) \\
    \hdots \\
    C \leadsto C' &\Rightarrow& \kw{typecase}~C~\kw{of}\ (M_B, M_I, M_S, \beta.M_L, \rho.M_R, \gamma.M_T) &\leadsto \kw{typecase}~C'~\kw{of}\ (M_B, M_I, M_S, \beta.M_L, \rho.M_R, \gamma.M_T)  \\
    M_B \leadsto M_B' &\Rightarrow& \kw{typecase}~C~\kw{of}\ (M_B, M_I, M_S, \beta.M_L, \rho.M_R, \gamma.M_T) &\leadsto \kw{typecase}~C~\kw{of}\ (M_B', M_I, M_S, \beta.M_L, \rho.M_R, \gamma.M_T)  \\
    \hdots \\
  \end{align*}

  \caption{Congruence rules allow subterms to reduce independently.}% See also $\beta$-rules and commuting conversions in Figure \ref{fig:normalization-rules} and constructor computation in Figure \ref{fig:constructor-computation}.}
  \label{fig:normalization-rules-congruence}
\end{figure*}

\subsection{Proof of Lemma~\ref{lem:preservation-constructor}}
\begin{proof}
  By induction on the kinding derivation.
  We look at the possible reductions (see Figure \ref{fig:constructor-computation}).
  Congruence rules allow for reduction in rows, function bodies, applications, list, trace, record, row map, and typerec. These all follow directly from the induction hypothesis.
  The remaining cases are:
  \begin{itemize}
  \item $(\lambda\alpha:K.C)\ D \leadsto C[\alpha \coloneqq D]$: by Lemma \ref{lem:substitution-lemmas}.
  \item $\kw{Rmap}\ C\ \cdot \leadsto \cdot$: both sides have kind \textit{Row}.
  \item $\kw{Rmap}\ C\ (l:D; S) \leadsto (l: C\ D; \kw{Rmap}\ C\ S)$: from the induction hypothesis we have that
    $C$ has kind $\mathit{Type} \rightarrow \mathit{Type}$,
    $D$ has kind $\mathit{Type}$, and $S$ has kind \textit{Row}.
    Therefore $C\ D$ has kind \textit{Type} and the whole right-hand side has kind \textit{Row}.
  \item Typerec $\beta$-rules:
    \begin{itemize}
    \item Base type right hand sides have kind \textit{Type} by IH.
    \item List left-hand side
      $ \kw{Typerec}~\texttt{List}^*~D~(C_B, C_I, C_S, C_L, C_R, C_T)
      $ and right-hand side
      $ C_L\ D\ (\kw{Typerec}~D~(C_B, C_I, C_S, C_L, C_R, C_T))$:

      $C_L$ has kind $\mathit{Type} \rightarrow K \rightarrow K$ by IH. $D$ has kind \textit{Type} by IH, and the typerec expression has kind $K$.

    \item Record left-hand side
      $ \kw{Typerec}~\texttt{Record}^*~S~(C_B, C_I, C_S, C_L, C_R, C_T) $
      and right-hand side
      $ C_R\ S\ (\kw{Rmap}\ (\lambda \alpha.\kw{Typerec}~\alpha~(C_B, C_I, C_S, C_L, C_R, C_T))\ S) $:

      $C_L$ has kind $\mathit{Row} \rightarrow \mathit{Row} \rightarrow K$ by IH.
      $S$ has kind \textit{Row} by IH.
      The row map expression has kind \textit{Row}, because the type-level function has kind $\mathit{Type} \rightarrow \mathit{Type}$.

    \item The trace case is analogous to the list case.
      \qedhere
    \end{itemize}
  \end{itemize}
\end{proof}

\subsection{Proof of Lemma~\ref{lem:preservation}}
\begin{proof} By induction on the typing derivation $\Gamma \vdash M : A$.
  Constants, variables, empty lists, and empty records do not reduce.
  We omit discussion of the cases that follow directly from the induction hypothesis, Lemma \ref{lem:preservation-constructor}, and congruence rules (see Figure \ref{fig:normalization-rules-congruence}), like $M + N$ being able to reduce in both $M$ and~$N$.
  The remaining, interesting reduction rules are the $\beta$-rules in Figure~\ref{fig:normalization-beta} and the commuting conversions in Figure~\ref{fig:normalization-cc}.
  We discuss them grouped by the relevant typing rule.
  \begin{itemize}
  \item Function application:
    \begin{itemize}
    \item $(\lambda x.M)\ N \leadsto M[x \coloneqq N]$: follows from Lemma \ref{lem:substitution-lemmas}.
    \item $(\kw{if}~L~\kw{then}~M_1~\kw{else}~M_2)\ N \leadsto \kw{if}~L~\kw{then}~M_1\ N~\kw{else}~M_2\ N$:

      We have: \[\footnotesize
        \infer*
        { \infer*
          { Γ ⊢ L : \mathtt{Bool} \and Γ ⊢ M_1 : A \rightarrow B \and Γ ⊢ M_2 : A \rightarrow B}
          { Γ ⊢ \kw{if}~L~\kw{then}~M_1~\kw{else}~M_2 : A \rightarrow B } \and Γ ⊢ N : A }
        { Γ ⊢ (\kw{if}~L~\kw{then}~M_1~\kw{else}~M_2)\ N : B }
      \]
      and can therefore show: \[\footnotesize
        \infer*
        { Γ ⊢ L : \mathtt{Bool} \and
          \infer* { Γ ⊢ M_1 : A \rightarrow B \and Γ ⊢ N : A } { Γ ⊢ M_1\ N : B } \and
          \infer* { Γ ⊢ M_2 : A \rightarrow B \and Γ ⊢ N : A } { Γ ⊢ M_2\ N : B }
        }
        { Γ ⊢ \kw{if}~L~\kw{then}~M_1\ N~\kw{else}~M_2\ N : B }
      \]
    \end{itemize}

  \item Type instantiation:
    \begin{itemize}
    \item $(\Lambda \alpha.M)\ C \leadsto M[\alpha \coloneqq C]$: follows from the constructor substitution lemma (Lemma \ref{lem:substitution-lemmas}). % \stefan{could expand on this with more rules..}
    \item $(\kw{if}~L~\kw{then}~M_1~\kw{else}~M_2)\ C \leadsto \kw{if}~L~\kw{then}~M_1\ C~\kw{else}~M_2\ C$: hoisting if-then-else out of the term works the same as application above.
    \end{itemize}

  \item Fixpoint: follows from the substitution lemma (Lemma \ref{lem:substitution-lemmas}).
  \item If-then-else: if the condition is a Boolean constant, the expression reduces to the appropriate branch, which has the correct type by IH.
    The commuting conversion for lifting if-then-else out of the condition is type-correct by IH and rearranging of if-then-else rules.
  \item List comprehensions:
    \begin{itemize}
    \item The if-then-else commuting conversion is as before.
    \item $\kw{for}~(x \leftarrow [])~N \leadsto []$: $[]$ has any list type and $N$ has a list type.
    \item $ \kw{for}~(x \leftarrow [M])~N \leadsto N[x \coloneqq M] $: by substitution (Lemma \ref{lem:substitution-lemmas}).
    \item $ \kw{for}~(x \leftarrow M_1 \concat M_2)~N \leadsto (\kw{for}~(x \leftarrow M_1)~N) \concat (\kw{for}~(x \leftarrow M_2)~N) $: reorder rules.
    \item $\kw{for}~(x \leftarrow \kw{for}~(y \leftarrow L)~M)~N \leadsto \kw{for}~(y \leftarrow L)~\kw{for}~(x \leftarrow M)~N $:

      We have:
      \[ \infer*
        { \infer*
          { Γ ⊢ L : [A_L] \\
            Γ, y:A_L ⊢ M : [A_M] }
          { Γ ⊢ \kw{for}~(y \leftarrow L)~M : [A_M]
          } \and Γ,x:A_M ⊢ N : [A_N]
        }
        { Γ ⊢ \kw{for}~(x \leftarrow \kw{for}~(y \leftarrow L)~M)~N : [A_N] }
      \]

      We need:
      \[ \infer*
        { Γ ⊢ L:[A_L] \and
          \infer*
          { Γ, y:A_L ⊢ M:[A_M] \and
            Γ, y:A_L, x:A_M ⊢ N : [A_N] }
          { Γ, y:A_L ⊢ \kw{for}~(x \leftarrow M)~N : [A_N] }
        }
        { Γ ⊢ \kw{for}~(y \leftarrow L)~\kw{for}~(x \leftarrow M)~N : [A_N] }
      \]

      We obtain $Γ, y:A_L, x:A_M ⊢ N : [A_N]$ from $Γ,x:A_M ⊢ N : [A_N]$ by weakening (Lemma \ref{lem:weakening}) and context swap (Lemma \ref{lem:context-swap}).
    \end{itemize}

  \item Projection: The $\beta$ rule is obvious, the if-then-else commuting conversion is as before.

  \item Type equality $\infer { Γ ⊢ N : B \\ Γ ⊢ A = B } { Γ ⊢ N : A }$: for all $N'$ with $N \leadsto N'$ we have that $\Gamma \vdash N' : B$ by the induction hypothesis. We also know that $Γ ⊢ A = B$, so $\Gamma \vdash N' : A$ by this typing rule and symmetry of type equality.

  \item Case \kw{rmap}:
    Typing rule:
    \[    \infer
      { Γ ⊢ M : \forall \alpha: \textit{Type}. \texttt{T}(\alpha) \rightarrow \texttt{T}(C\ \alpha) \\
        Γ ⊢ N : \texttt{T}(\texttt{Record}^*\ S)}
      { Γ ⊢ \kw{rmap}^S~M~N : \texttt{T}(\texttt{Record}^*\ (\kw{Rmap}\ C \ S))}
    \]
    Reduction rule:
    \[
      \kw{rmap}^{\langle \overline{l_i:C_i}  \rangle}\ M\ N
      \leadsto \langle \overline{l_i = (M\ C_i)\ N.l_i } \rangle
    \]
    Need to show that $\langle \overline{l_i = (M\ C_i)\ N.l_i } \rangle : \texttt{T}(\texttt{Record}^*\ (\kw{Rmap}\ C \ \langle \overline{l_i:C_i}  \rangle))$.
    By row type constructor evaluation, that type equals $\texttt{T}(\texttt{Record}^*\ \langle \overline{l_i:C\ C_i}  \rangle)$, which is the obvious type of $\langle \overline{l_i = (M\ C_i)\ N.l_i } \rangle$.

  \item Case \kw{rfold}:     Typing rule:
    \[    \infer
    { Γ ⊢ L: \texttt{T}(C) \rightarrow \texttt{T}(C) \rightarrow \texttt{T}(C) \\
      Γ ⊢ M : \texttt{T}(C) \\
      Γ ⊢ N : \texttt{T}(\texttt{Record}^*\ (\kw{Rmap}\ (\lambda\alpha.\alpha \rightarrow C)\ S)) }
    { Γ ⊢ \kw{rfold}^S\ L\ M\ N:\texttt{T}(C) }
  \]
  Reduction rule:
  \[
    \kw{rfold}^{(\overline{l_i: C_i})}\ L\ M\ N \leadsto L\ N.l_1\ (L\ N.l_2 \hdots (L\ N.l_n\ M) \hdots)
  \]
  Need to show that $L\ N.l_1\ (L\ N.l_2 \hdots (L\ N.l_n\ M) \hdots)$ has type \lstinline|T($C$)|.
  $M$ has type \lstinline|T($C$)|.
  $L$ has type $\texttt{T}(C) \rightarrow \texttt{T}(C) \rightarrow \texttt{T}(C)$.
  Each $N.l_i$ has type \lstinline|T($C$)|, because $N$ has a record type obtained by mapping the constant function with result $C$ over row $S$.

  \item Typecase typing rule:
    \[ \infer
      { Γ ⊢ C : \textit{Type} \\
        Γ, \alpha: \textit{Type} ⊢ B : \textit{Type} \\
        \beta, \rho, \gamma \notin \textit{Dom}(Γ) \\
        Γ ⊢ M_B : B[\alpha \coloneqq \texttt{Bool}^*] \\
        Γ ⊢ M_I : B[\alpha \coloneqq \inttyc] \\
        Γ ⊢ M_S : B[\alpha \coloneqq \texttt{String}^*] \\
        Γ, \beta : \textit{Type} ⊢ M_L : B[\alpha \coloneqq \texttt{List}^*\ \beta] \\
        Γ, \rho : \textit{Row} ⊢ M_R : B[\alpha \coloneqq \texttt{Record}^*\ \rho] \\
        Γ, \gamma : \textit{BaseType} ⊢ M_T : B[\alpha \coloneqq \texttt{Trace}^*\ \gamma]
      }
      { Γ ⊢ \kw{typecase}^{\alpha.B}~C~\kw{of}\ (M_B, M_I, M_S, \beta.M_L, \rho.M_R, \gamma.M_T) : B[\alpha \coloneqq C] } \]

    Reduction rules:
    \begin{itemize}
    \item $\kw{typecase}~\texttt{Bool}^*~\kw{of}\ (M_B, M_I, M_S, \beta.M_L, \rho.M_R, \gamma.M_T) \leadsto M_B$

      Need to show that $M_B:B[\alpha \coloneqq \texttt{Bool}^*]$, which is one of our hypotheses.
    \item $\kw{typecase}~\texttt{List}^*~C~\kw{of}\ (M_B, M_I, M_S, \beta.M_L, \rho.M_R, \gamma.M_T) \leadsto M_L[\beta \coloneqq C]$

      Need to show that the result of reduction $M_L[\beta \coloneqq C]$ has type $B[\alpha \coloneqq \texttt{List}^*\ C]$, the same as the typing rule.

      \[
        \infer { }
        { \Gamma \vdash M_L[\beta \coloneqq C] : B[\alpha \coloneqq \texttt{List}^*\ C] }
      \]

      Instantiating the constructor substitution lemma (Lemma \ref{lem:substitution-lemmas}) gives us
      \[ \Gamma[\beta \coloneqq C] \vdash M_L[\beta \coloneqq C] : (B[\alpha \coloneqq \texttt{List}\ \beta])[\beta \coloneqq C]
      \]
      from $\Gamma, \alpha: \mathit{Type} \vdash B: \mathit{Type}$ and $\beta \notin \textit{Dom}(Γ)$ we know that neither $B$ nor $\Gamma$ can contain $\beta$.
      Thus the only substitution for $\beta$ we need to perform is in the substitution for $\alpha$ and we can reassociate substitution like this:
      \[ \Gamma \vdash M_L[\beta \coloneqq C] : B([\alpha \coloneqq \texttt{List}\ \beta][\beta \coloneqq C])
      \]
      which is the same as
      \[ \Gamma \vdash M_L[\beta \coloneqq C] : B[\alpha \coloneqq \texttt{List}\ C] \]
    \end{itemize}
    The other cases are analogous.

  % \item Trace constructors: by IH and \stefan{preservation of constructor reduction TODO that's the version of preservation for constructors, not a substitution lemma}.
  \item Case \lstinline|tracecase|: Typing rule: {\footnotesize \[    \infer
        { Γ ⊢ M : \texttt{Trace}\ A \\
          Γ, x_L : A ⊢ M_L : B \\
          Γ, x_I : \langle\mathsf{cond}: \texttt{Trace}\ \texttt{Bool}, \mathsf{then}: \texttt{Trace}\ A\rangle ⊢ M_I : B \\
          Γ, \alpha_F: \textit{Type}, x_F : \langle\mathsf{in}: \texttt{T}(\texttt{TRACE}\ \alpha_F), \mathsf{out}: \texttt{Trace}\ A\rangle ⊢ M_F : B \\
          Γ, x_C : \langle\mathsf{table}: \texttt{String}, \mathsf{column}: \texttt{String}, \mathsf{row}: \intty, \mathsf{data} : A\rangle ⊢ M_C : B \\
          Γ, \alpha_E : \textit{Type}, x_E : \langle\mathsf{left}: \texttt{T}(\texttt{TRACE}\ \alpha_E), \mathsf{right}: \texttt{T}(\texttt{TRACE}\ \alpha_E)\rangle ⊢ M_E : B \\
          Γ, x_P : \langle\mathsf{left}: \texttt{Trace}\ \intty, \mathsf{right}: \texttt{Trace}\ \intty\rangle ⊢ M_P : B \\
        }
        { Γ ⊢ \kw{tracecase}~M~\kw{of}\ (x_L.M_L, x_I.M_I, \alpha_F.x_F.M_F, x_C.M_C, \alpha_E.x_E.M_E, x_P.M_P) : B }
      \]}

    Reductions:
    \begin{itemize}
    \item $ \kw{tracecase}~\texttt{For}~C~M~\kw{of}\ (x.M_L, x.M_I, \alpha.x.M_F, x.M_C, \alpha.x.M_E, x.M_P) \leadsto M_F[\alpha \coloneqq C, x \coloneqq M] $

      We need to show
      $\infer{\star}{\Gamma \vdash M_F[\alpha \coloneqq C, x \coloneqq M] : A}$

      $\star$: We only need $M: \langle \mathsf{in}: \dots \rangle$ and $C: \mathit{Type}$, which we get by inversion of the typing rule for \lstinline|For| and the substitution lemmas.
    \end{itemize}
    The other cases are analogous.
    \qedhere
  \end{itemize}
\end{proof}

\subsection{Proof of Lemma~\ref{lem:progress-constructor}}
\begin{proof}
  By induction on the kinding derivation of $C$ or $S$ (see Figure \ref{fig:constructor-formation}).
  \begin{itemize}
  \item Base types \texttt{Bool}, \intty, \texttt{String} are in normal form.
  \item Type variables $\alpha$ are in normal form.
  \item Type-level functions $\lambda \alpha.C$: by IH, either $C \leadsto C'$, in which case $\lambda \alpha.C \leadsto \lambda \alpha.C'$, or $C$ is in normal form already, in which case $\lambda \alpha.C$ is in normal form, too.
  \item Type-level application $C\ D$: by IH either $C$ or $D$ may reduce, in which case the whole application reduces. Otherwise, $C$ and $D$ are in normal form.
    The following cases of $C$ do not apply, because they are ill-kinded: base types, lists, records, and traces.
    If $C$ is a normal form and a variable, application, or typerec then $C$ is a neutral form and $D$ is a normal form so $C\ D$ is a neutral (and normal) form.
    Finally, if $C$ is a type-level function, the application $\beta$-reduces.
  \item List types: by IH either the argument reduces, or is in normal form already.
  \item Record types: by IH either the argument (a row) reduces, or is in normal form already.
  \item Trace types: by IH either the argument reduces, or is in normal form already.

  \item $\kw{Typerec}\ C\ \kw{of} (C_B, C_I, C_S, \alpha.C_L, \rho.C_R, \alpha.C_T)$: by IH, either $C \leadsto C'$, in which case \lstinline|Typerec| reduces with a congruence rule, or $C$ is in one of the following normal forms:
    \begin{itemize}
    \item If $C$ is a base, list, record, or trace constructor, the \lstinline|Typerec| expression $\beta$-reduces to the respective branch.
    \item $C$ cannot be a type-level function, that would be ill-kinded.
    \item If $C$ is one of the following neutral forms: variables, applications, and \kw{Typerec}, then by IH the branches $C_B$, $C_I$, etc. either reduce and a congruence rule applies, or they are all in normal form and $\kw{Typerec}\ C\ \kw{of} (C_B, C_I, C_S, \alpha.C_L, \rho.C_R, \alpha.C_T)$ is in normal form.
    \end{itemize}

% ROWS
% \james{These cases are a little handwavy, I would like to see a little more detail for the cases that are not as standard such as involving Typerec or Rmap}

  \item The empty row $\cdot$ is in normal form.
  \item Row extensions $l:C;S$: by IH applied to $C$ and $S$ we have three cases:
    \begin{itemize}
    \item If $C \leadsto C'$, then $l:C;S \leadsto l:C';S$.
    \item If $S \leadsto S'$, then $l:C;S \leadsto l:C;S'$.
    \item If $C$ and $S$ are in normal form, then $l:C;S$ is in normal form.
    \end{itemize}

  \item $\kw{Rmap}\ C\ S$: we apply the induction hypothesis to $S$ and $C$. If either $C$ or $S$ takes a step, the whole row map expression takes a step via the respective congruence rule.
    Otherwise $S$ is in one of the following normal forms:
    \begin{itemize}
    \item Case empty row: $\kw{Rmap}\ C\ \cdot \leadsto \cdot$
    \item Case $l:D;S'$: $\kw{Rmap}\ C\ (l:D;S') \leadsto (l:C\ D; \kw{Rmap}\ C\ S')$.
    \item Case $\kw{Rmap}\ D\ U$: $\kw{Rmap}\ C\ (\kw{Rmap}\ D\ U)$ is in normal form.
    \item Case $\rho$: $\kw{Rmap}\ C\ \rho$ is in normal form.
    \end{itemize}
  \item The row variable $\rho$ is in normal form.
    \qedhere
  \end{itemize}
\end{proof}

\subsection{Proof of Lemma~\ref{lem:progress}}
\begin{proof} By induction on the typing derivation of $M$.

\begin{itemize}
\item Constants: in normal form.
\item Term variables: in normal form.
\item Term function: apply IH to body and either reduce or in normal form.
\item Fixpoint: we can always take a step by unrolling once.

\item Term application $M\ N$: apply induction hypothesis to $M$. If $M$ reduces to $M'$, then $M\ N$ reduces to $M'\ N$. Otherwise, $M$ is in \TLinks normal form. It cannot be any of the following, because these would be ill-typed: constants, type abstraction, operators, record introduction forms including record map, list introduction forms, trace introduction forms.
  % \james{This reasoning can be made clearer by considering all the possible well-typed normal forms M (something of function type) could have.  It might be helpful to split this reasoning out into a separate lemma, saying for each type (or type constructor) what the normal forms it can have look like.} \stefan{I've had something like that before. I'm not sure it's better. It certainly is longer: it takes a page per lemma instead of a paragraph.}
  In the following cases, we apply the induction hypothesis to $N$ and either reduce to $M\ N'$ or are in normal form already: variable, application, type application, record fold, tracecase, typecase.
  This leaves the following cases:
  \begin{itemize}
  \item If $M$ is a function, we $\beta$-reduce.
  \item If $M$ is of the form if-then-else, we reduce using a commuting conversion.
  \end{itemize}

\item Term-level type abstraction $\forall \alpha:M$: by IH, either $M \leadsto M'$, in which case $\forall \alpha:M \leadsto \forall \alpha:M'$, or $M$ is in normal form, in which case $\forall \alpha:M$ is in normal form as well.

\item Term-level type application $M\ C$: apply induction hypothesis to $M$. If $M$ reduces to $M'$, then $M\ C$ reduces to $M'\ C$. Otherwise, $M$ is in \TLinks normal form.
  It cannot be any of the following, because these would be ill-typed: constants, functions, operators, record introduction forms including record map, list introduction forms, trace introduction forms.
  In the following cases, the application is already in normal form: variable, application, type application, projection, record fold, tracecase, typecase.
  This leaves the following cases:
  \begin{itemize}
  \item If it is a term-level type abstraction, we $\beta$-reduce.
  \item If it is of the form if-then-else, we perform a commuting conversion.
  \end{itemize}

\item Case $\kw{if}~L~\kw{then}~M~\kw{else}~N$: apply induction hypothesis to all subterms.
  If any of the subterms reduce, then the whole if-then-else reduces.
  Otherwise, $L, M, N$ are in \TLinks normal form.
  The condition cannot be any of the following, because these would be ill-typed: functions, type abstractions, arithmetic operators, record introduction forms including record map, list introduction forms, trace introduction forms.
  In the following cases, the condition already matches the normal form: variable, application, type application, projection, record fold, tracecase, and typecase.
  This leaves the following cases for the condition:
  \begin{itemize}
  \item Constants: \lstinline|true| and \lstinline|false| reduce, other constants are ill-typed.
  % \item If it is a variable $x$, then $\kw{if}~x~\kw{then}~M~\kw{else}~N$ is in normal form.
  % \item If it is an application $F\ L'$, then $\kw{if}~F\ L'~\kw{then}~M~\kw{else}~N$ is in normal form.
  % \item If it is an application $G\ C$, then $\kw{if}~G\ C~\kw{then}~M~\kw{else}~N$ is in normal form.
  \item If the condition is of the form if-then-else itself, we apply a commuting conversion.
  \item Operators with Boolean result like \lstinline!==! are in normal form.
  \end{itemize}

\item Records $\langle l = M; N \rangle$: apply induction hypothesis to $M$ and $N$. If either reduces, the whole record reduces, otherwise it is in normal form.

\item Projection $M.l$: apply induction hypothesis to $M$. If $M$ reduces to $M'$, then $M.l$ reduces to $M'.l$. Otherwise, $M$ is in \TLinks normal form.
  It cannot be any of the following, because these would be ill-typed: constants, functions, type abstraction, operators, list introduction forms, trace introduction forms.
  In any of the following cases of $M$, $M.l$ is already in normal form: variable, application, type application, projection, record map, record fold, typecase, tracecase.
  This leaves the following cases for $M$:
  \begin{itemize}
  \item If it is of the form if-then-else itself, we apply a commuting conversion.
  \item It cannot be an empty record, or a record expression where label $l$ does not appear---these would be ill-typed. If $M$ is a record literal that maps $l$ to $M'$ then $\langle l = M'; N \rangle.l$ reduces to $M'$.
  \end{itemize}

\item Record map $\kw{rmap}^S\ M\ N$: by Lemma \ref{lem:progress-constructor} we have that either $S$ reduces to $S'$, in which case $\kw{rmap}^S\ M\ N$ reduces to $\kw{rmap}^{S'}\ M\ N$, or is in normal form. Similarly, $M$ and $N$ may reduce by IH. Otherwise, we have $S$, $M$, and $N$ in normal form. By cases of $S$:
  \begin{itemize}
  \item If it is a closed row, we apply the $\beta$-rule.
  \item If it is an open row $U$, $\kw{rmap}^U\ M\ N$ is in normal form.
  \end{itemize}

\item Record fold $\kw{rfold}^S\ L\ M\ N$: same as record map.
\item Empty list: in normal form.
\item Singleton list: apply IH to element and reduce or is in normal form.
\item List concatenation: apply IH to both sides. If either reduces, the whole concatenation reduces, otherwise it is in normal form.

\item Comprehension $\kw{for}~(x \leftarrow M)~N$: apply induction hypothesis to $M$. If $M$ reduces to $M'$ then $\kw{for}~(x \leftarrow M)~N$ reduces to $\kw{for}~(x \leftarrow M')~N$. Otherwise, $M$ is in \TLinks normal form. It cannot be any of the following, because these would be ill-typed: constants, functions, type abstractions, primitive operators, record introduction forms including record map, and trace constructors. In the following cases we apply the IH to the body and either reduce or the whole comprehension is in normal form: variables, term application, type application, projection, tables, record fold, tracecase, typecase. This leaves the following cases for $M$:
  \begin{itemize}
  \item If-then-else: reduces with a commuting conversion.
  \item Empty list: the whole comprehension reduces to the empty list.
  \item Singleton list: $\beta$-reduces.
  \item List concatenation: reduces with a commuting conversion.
  \item Comprehension: reduces with a commuting conversion.
  \end{itemize}
\item Table: in normal form.
\item Trace constructors: apply IH and Lemma~\ref{lem:progress-constructor} to constituent parts. If either reduces, the whole trace constructor reduces, otherwise it is in normal form.

\item Tracecase: apply induction hypothesis to the scrutinee. If it reduces, the whole tracecase expression reduces. Otherwise it is in \TLinks normal form.
  It cannot be any of the following, because these would be ill-typed:
  constants, functions, type abstractions, primitive operators, record introduction forms, record map, empty or singleton lists, list concatenations or comprehensions, tables.
  If the scrutinee is any of the following, by IH we reduce in the branches or the whole tracecase is in normal form: variables, term application, type application, projection, record fold, tracecase, typecase.
  This leaves the following cases:
  \begin{itemize}
  \item If-then-else: reduces using commuting conversion.
  \item Trace constructor: $\beta$-reduces.
  \end{itemize}

\item Typecase: apply Lemma~\ref{lem:progress-constructor} to the scrutinee.
  Either it reduces, in which case the whole typecase expression reduces.
  Otherwise it is in normal form.
  It cannot be a type-level function, that would be ill-kinded.
  In the following cases, we apply the induction hypothesis to the branches of the typecase and reduce there, or we are in \TLinks normal form: type variables, type-level application, and typerec.
  And finally, if the outmost constructor is one of the following, a $\beta$-rule applies: bool, int, string, list, record, trace.

\item Primitive operators like \lstinline!==! and \lstinline|+|: by IH either the arguments reduce, in which case the whole expression reduces, or are in normal form, in which case the whole expression is in normal form.
  \qedhere
\end{itemize}
\end{proof}

\subsection{Proof of Lemma~\ref{lem:f-collapses}}
\begin{proof}
  By induction on the typing derivation.
  The term cannot be a record fold or typecase, because those necessarily contain a (row) type variable, which is unbound in the query context $\Gamma$.
  It cannot be a term application, type application, or tracecase, because the term in function position or the scrutinee, by IH, is of the form $x$ or $x.l$, both of which are ill-typed given that the query context $\Gamma$ does not contain function types, polymorphic types, or trace types.
  Projections $P.l$ are of the form $F.l$ or $(\kw{rmap}^U\ M\ N).l$.
  The former case reduces by IH to $x.l$ or $x.l'.l$, the first of which is okay, and the second is ill-typed.
  The latter case is impossible, because $U$ necessarily contains a row variable and would therefore be ill-typed.
  This leaves variables $x$ and projections of variables $x.l$.
\end{proof}

\subsection{Proof of Theorem~\ref{thm:nf-query-nrc}}
\begin{proof} By induction on the typing derivation.
  \begin{itemize}
  \item Constants, variables, empty lists, and tables are in both languages.
  \item Functions, type abstractions, and trace constructors do not have nested relational type.
  \item Function application:
    The typing rule
    \[ \infer
      { Γ ⊢ M': A \rightarrow B \\ Γ ⊢ N: A }
      { Γ ⊢ M' N : B } \]
    requires $M'$ to have a function type.
    Since $M$ is in normal form, $M'$ matches the grammar $F$.
    Lemma~\ref{lem:f-collapses} implies that $M'$ is either a variable $x$ or a projection $x.l$.
    The query context $\Gamma$ assigns record types with labels of base types to all variables --- not function types --- a contradiction.
    % $M$ cannot be an application without violating at least one of the constraints.

  \item Type instantiation:
    The typing rule
    \[ \infer
      { Γ ⊢ M': \forall \alpha:K.A \\ Γ ⊢ C: K}
      { Γ ⊢ M'\ C : A[\alpha \coloneqq C]} \]
    requires $M'$ to have a polymorphic type.
    The normal form assumption requires $M'$ to match the normal form $F$.
    Therefore, Lemma~\ref{lem:f-collapses} applies, so $M'$ is either a variable $x$ or a projection $x.l$.
    The query context $\Gamma$ assigns record types with labels of base types to all variables --- a contradiction.

  \item Primitive operators, if-then-else, records, singleton list, and list concatenation: apply the induction hypothesis to the subterms.
  % \item +: IH.
  % \item ==: IH.
  % \item Records: IH.
  \item Projection $M'.l$: $M'$ is in normal form $P$, which is either of the form $F$ or a record map.
    Lemma \ref{lem:f-collapses} restricts $F$ to $x$ and $x.l'$, both of which are nested relational calculus terms.
    $P$ cannot be of the form $\kw{rmap}^U\ N'\ N''$, because $U$ necessarily contains a free type variable (see Remark \ref{remark:constructors-free-type-variable}), and thus cannot be well-typed in a query context $\Gamma$ which does not contain type variables.

  \item Record map and fold have normal forms $\kw{rmap}^U\ M'\ N$ and $\kw{rfold}^U\ L\ M'\ N$, respectively.
    $U$ necessarily contains a free type variable (see Remark \ref{remark:constructors-free-type-variable}), and thus cannot be well-typed in a query context $\Gamma$ which does not contain type variables.

  \item List comprehension $\kw{for}\ (x \leftarrow M')\ N$:
    The iteratee $M'$ is in normal form $T$, which includes tables and normal forms $F$.
    If $M'$ is a table, $x$ has closed record type with labels of base types, the induction hypothesis applies to $N$, and the whole expression is in nested relational calculus.
    If $M'$ is of the form $F$, Lemma~\ref{lem:f-collapses} applies and implies that $M'$ is either $x$ or $x.l$.
    Both cases are ill-typed, because the query context $\Gamma$ only contains variables with closed records with labels of base type --- a contradiction.

  \item Tracecase: much like the application case above, the typing derivation forces the scrutinee to be of trace type.
    The normal form forces the scrutinee to be of the form $F$, and from Lemma \ref{lem:f-collapses} follows that it has to be a variable, or projection of a variable.
    The query context $\Gamma$ assigns record types with labels of base types to all variables --- a contradiction.

  \item Typecase: the scrutinee is in normal form $E$ which contains at least one free type variable (see Remark \ref{remark:constructors-free-type-variable}).
    In a query context which only binds term variables, this cannot possibly be well-typed --- a contradiction.
    \qedhere
  \end{itemize}
\end{proof}
